# Supplementary material for: Transformer Vs. MLP-Mixer: Exponential Expressive Gap For NLP Problems
Source: arXiv:2208.08191 source file (2022-11-17)
Supplement: Supplementary file 2 [file appendix_A.tex]

\section{Separation-rank upper bounds}
\begin{definition}
    Let $f:\mathcal{X}^M \to \mathbb{R}^{n \times m}$ be some function. 
    With
    \equ{
        \sup-sep-rank\lb f\rb=\inf-sep-rank\lb f\rb
    }
    Then the $sep-rank$  of $f$ exists. And is defined 
    to be 
    \equ{
        sep-rank\lb f\rb \defeq \sup-sep-rank\lb f\rb = \inf-sep-rank\lb f\rb
    }
\end{definition}

\subsection{Lemma 5.1}
\begin{lemma}\label{lem_547}
    Let $\;f,\; g: \mathbb{R}^{k \times l} \,\to\, \mathbb{R}^{n \times m}\;$, 
    be a matrix functions. And let $\;k_f \defeq sep-rank\lb f\lb X\rb\rb\;$
    be the separation-rank of $f$. Then we have the following properties
    \begin{adjustwidth}{1cm}{}
        \begin{description}
           \item[(i)] Separation rank is a sub-additive operator
                \equ{\label{lem24}
                    sep-rank\lb f\lb X\rb + g\lb X\rb \rb 
                    \leq 
                    sep-rank\lb f\lb X\rb\rb  + sep-rank\lb g\lb X\rb \rb  
                }    
                \item[(ii)]\label{permu_lemma} Separation-rank, is invariant under permutations. And more formally  
                let $\pi \in S_{n \cdot m}$ be a permutation over the entries of 
                $\;n \times m\;$ matrices. And let $f: \mathbb{R}^{k \times l} \to \mathbb{R}^{n \times m}$ be a matrix function. Then the following equality holds  
                \equ{
                    sep-rank\lb \pi \circ f\lb X\rb\rb = sep-rank\lb f\lb X\rb\rb 
                }
                \item[(iii)] \label{lem218}
                For $Id: M_{n \times m}\lb \mathbb{R}\rb \to M_{n \times m}\lb \mathbb{R}\rb$ we have
                \equ{
                    sep-rank\lc Id\lb X\rb\rc \leq 2 
                }   
            \item[(iv)] \label{lem22} 
            The following inequality holds
            \equ{
                sep-rank\lb f\lb X\rb^{\odot 2}\rb
                \,\leq\,  
                \binom{k_f+1}{2}
            }
            Where $\odot$ is the Hadmard product. And is defined by  
            $\,\lb A^{\odot k}\rb_{i j} = \lb A_{i j}\rb^k$.
            %\item[(v)] \label{lem21}
            %    For every matrix $W\in \mathbb{R}^{r \times n}$,
            %    we have 
            %    \equ{
            %        sep-rank\lb W f\lb X\rb\rb \leq n \cdot sep-rank\lb f\lb     % X\rb\rb 
            %}
        \end{description}
    \end{adjustwidth}
\end{lemma}

\begin{proof}
    The claims will be proven, one by one, according for their order in the lemma.
    \begin{adjustwidth}{1cm}{}
        \begin{description}
            \item[(i)] \label{proof_216}
                        Denote $k_f = sep-rank\lb f\rb$ and $k_g = sep-rank\lb g\rb$ then 
                    \begin{align*}
                        \exists \;\phi_1, ..., \phi_{k_f}, \psi_1, ..., \psi_{k_f}, 
                                \xi_1, ..., \xi_{k_g}, \zeta_1, ..., \zeta_{k_g}: 
                                Domain\lc f\rc \to Range\lc f\rc
                    \end{align*}
                    s.t
                    \begin{align*}
                        f\lb X\rb = \overset{k_f}{\underset{i=1}{\Sigma}}\;  \phi_i\lb X_A\rb \odot \psi_i\lb X_B\rb
                        \quad\quad\bigwedge\quad\quad
                        g\lb X\rb = \overset{k_g}{\underset{i=1}{\Sigma}}\;  \xi_i\lb X_A\rb \odot \zeta_i\lb X_B\rb                        
                    \end{align*}
                    In particular
                    \begin{align*}
                        f\lb X\rb + g\lb X\rb
                         = 
                        \overset{k_f}{\underset{i=1}{\Sigma}}\;  \phi_i\lb X_A\rb \odot \psi_i\lb X_B\rb
                         + 
                        \overset{k_g}{\underset{i=1}{\Sigma}}\;  \xi_i\lb X_A\rb \odot \zeta_i\lb X_B\rb
                    \end{align*}
                    Is valid decomposition for $f+g$ with $k_f + k_g$ elements, and hence we have 
                    \begin{align*}
                        sep-rank\lb f\lb X\rb + g\lb X\rb \rb 
                        \leq 
                        sep-rank\lb f\lb X\rb\rb  + sep-rank\lb g\lb X\rb \rb
                    \end{align*}
                    As needed  \QED    
            \item[(ii)]  \label{proof_217}
                And indeed we have 
                \begin{align*}
                    &   sep-rank\lb \pi \circ f\lb X\rb\rb
                    = \underset{i,\, j \in \lc n\rc\times \lc m\rc}{\max}\;\,
                       \lb\, \pi \circ f\lb X\rb\,\rb_{i,\, j}
                    \\ &\quad
                    = \underset{i,\, j \in \lc n\rc\times \lc m\rc}{\max}\;\,
                       \lb\, f\lb X\rb\,\rb_{i,\, j}
                    = sep-rank\lb f\lb X\rb\rb 
                \end{align*}
            \item[(iii)] \label{proof_218}
                    The following is decomposition of order $2$
                    \begin{align*}
                        Id\lb X\rb = X = X_A + X_B =  X_A \odot \mathbf{1}_{n \times m} \,+\, \mathbf{1}_{n \times m} \odot X_B
                    \end{align*}
                    Where $\mathbf{1}_{n\times m}$ is the $n\times m$ matrix with all its entries $1$.$\quad\quad\blacksquare$     
            \item[(iv)] \label{proof_22}
                    We will show the more general claim, that for every $k\in \mathbb{N}$  it holds that 
                    \begin{align*}
                        sep-rank\lb f\lb X\rb^{\odot k}\rb \leq  \binom{k+k_f-1}{k}
                    \end{align*}
                    and the claim of the lemma will follow as particular case, by for $k=2$. So let
                    \begin{align*}
                        f\lb X\rb = \overset{k_p}{\underset{i=1}{\Sigma}} f_i\lb X_A\rb \odot g_i\lb X_B\rb
                    \end{align*}
                    be the promised decomposition of $f$ then we have 
                    \begin{align*}
                        & f\lb X\rb^{\odot k}
                        = 
                            \lb 
                                \overset{k_f}{\underset{i=1}{\Sigma}} f_i\lb X_A\rb \odot g_i\lb X_B\rb 
                            \rb^{\odot k}
                        \\ &
                        =  
                            \underset{i_1 + ... + i_{k_f}=k}{\Sigma}\; 
                            \binom{k_p}{i_1, ..., i_{k_f}}\;
                            \overset{p}{\underset{j=1}{\odot}}\;\lc 
                            f_i\lb X_A\rb^{\odot i_j}
                            \odot 
                            g_i\lb X_B\rb^{\odot i_j}\rc 
                            \\ &
                            = 
                            \underset{i_1 + ... + i_{k_f}=k}{\Sigma}\;
                            \binom{k_f}{i_1, ..., i_{k_f}}\;
                            \lb \overset{f}{\underset{j=1}{\odot}}\; f_i\lb X_A\rb^{\odot i_j} \rb
                            \odot 
                            \lb \overset{f}{\underset{j=1}{\odot}}\; g_i\lb X_B\rb^{\odot i_j} \rb
                    \end{align*}
                    Hence 
                    \begin{align*} 
                        sep-rank\lb f\lb X\rb^{\odot k}\rb \leq \underset{i_1 + ... + i_{k_f}=k}{\Sigma}\; 1
                        = \binom{k+k_f-1}{k_f-1} = \binom{k+k_f-1}{k}
                    \end{align*}
                    As we wanted \QED
        \end{description}
    \end{adjustwidth}
\end{proof}

\subsection{Some more separation-rank upper bounds}
\begin{lemma}\label{lem_548}
    Let $\;h,\; u: \mathbb{R}^{k \times l} \,\to\, \mathbb{R}\;$ 
    and $\;f,\; g: \mathbb{R}^{k \times l} \,\to\, \mathbb{R}^{n \times m}\;$
    be some scalar value and matrix value functions.
   Then we have the following properties
    \begin{adjustwidth}{1cm}{}
        \begin{description}
           \item[(i)] \label{lem225}
                    $separation-rank$ is invariant under the transpose operation  
                    \equ{
                        sep-rank\lb f\lb X\rb \rb \,=\, sep-rank\lb f\lb X\rb^T \rb
                    }    
            \item[(ii)] \label{lem212}
                 $separation-rank$ is sub-multiplicative, for scalar valued functions
                    \equ{
                        sep-rank\lb h\lb X\rb \cdot u\lb X\rb \rb \leq sep-rank\lb h\lb X\rb\rb \cdot sep-rank\lb u\lb X\rb\rb  
                    }
            \item[(iii)]\label{lem214}
                    $separation-rank$ is sub-multiplicative, up to dimension dependent constant 
                    for matrix valued functions
                    \equ{
                        sep-rank\lc f\lb X\rb \cdot g\lb X\rb\rc
                        \;\leq\; 
                        n \cdot sep-rank\lc f\lb X\rb\rc 
                        \cdot sep-rank\lc g\lb X\rb\rc 
                    }    
            \item[(iv)] \label{lem21}
                For every matrix $W\in \mathbb{R}^{r \times n}$ we have 
                \equ{
                    sep-rank\lb W f\lb X\rb\rb \leq n \cdot sep-rank\lb f\lb X\rb\rb 
                }
        \end{description}
    \end{adjustwidth}
\end{lemma}
\begin{proof} 
    The claims will be proven, one by one, according for their order in the lemma.
    \begin{adjustwidth}{1cm}{}
        \begin{description}
           \item[(i)] 
                    Using the $sep-rank$ definition we get 
                    \begin{align*}
                        & sep-rank\lb f\lb X\rb\rb
                        \,=\, \sup-sep\lb f\lb X\rb\rb
                        \\ & 
                        \underbrace{=\;\;}_\textit{definition} 
                        \underset{i, j}{\max} \, \lb 
                        \sup-sep\lc f\lb X\rb\rc_{i, j}\rb 
                        \,=\, \underset{j, i}{\max} \, \lb 
                        \sup-sep\lc f\lb X\rb\rc_{j, i}\rb
                        \\ & \quad\quad
                        =\, \underset{i, j}{\max} \, \lb 
                        \sup-sep\lc f\lb X\rb^T\rc_{i, j}\rb
                        \,=\,
                        \sup-sep\lb f\lb X\rb^T\rb
                        \quad\quad\quad\quad
                        \\ & 
                        \underbrace{\,=\,}_\textit{definition}
                        sep-rank\lb f\lb X\rb^T\rb \quad\quad\blacksquare 
                    \end{align*}    
            \item[(ii)]
                        Let $k_f \defeq sep-rank\lb f\lb X\rb\rb$ and $k_g \defeq sep-rank\lb g\lb X\rb\rb$ and let 
                    \begin{align*}
                        f\lb X\rb = \overset{k_f}{\underset{i=1}{\Sigma}}\;  \phi_i\lb X_A\rb \cdot \psi_i\lb X_B\rb
                        \quad\quad\bigwedge\quad\quad
                        g\lb X\rb = \overset{k_g}{\underset{i=1}{\Sigma}}\;  \xi_i\lb X_A\rb \cdot \zeta_i\lb X_B\rb
                    \end{align*}
                    be a corresponding decomposition's for $f,\, g$ then we have 
                    \begin{align*}
                        & f\lb X\rb \cdot g\lb X\rb
                         = 
                        \lc \overset{k_f}{\underset{i=1}{\Sigma}}\;  \phi_i\lb X_A\rb \cdot \psi_i\lb X_B\rb\rc 
                         \cdot
                        \lc \overset{k_g}{\underset{i=1}{\Sigma}}\;  \xi_i\lb X_A\rb \cdot \zeta_i\lb X_B\rb\rc
                        \\ & 
                        =
                        \overset{k_f}{\underset{i=1}{\Sigma}}\; \overset{k_g}{\underset{i=1}{\Sigma}}\;
                        \phi_i\lb X_A\rb \cdot \psi_i\lb X_B\rb \cdot 
                         \xi_i\lb X_A\rb \cdot \zeta_i\lb X_B\rb  
                        \\ & 
                        =
                        \overset{k_f}{\underset{i=1}{\Sigma}}\; \overset{k_g}{\underset{i=1}{\Sigma}}\;
                        \lc \phi_i\lb X_A\rb \cdot \xi_i\lb X_A\rb \rc 
                        \cdot 
                        \lc \psi_i\lb X_B\rb  \cdot \zeta_i\lb X_B\rb\rc      
                    \end{align*}
                    Hence, using the $sep-rank$ definition, we got  
                    \begin{align*}
                        sep-rank\lb f\lb X\rb \cdot g\lb X\rb \rb 
                        \;\leq\;
                        k_f \cdot k_g = sep-rank\lb f\lb X\rb\rb \cdot sep-rank\lb g\lb X\rb\rb
                    \end{align*}
                    as we wanted \QED
            \item[(iii)] 
                    Let fix some entry $i, j \in \lc n\rc \times \lc m\rc$ then 
                    \begin{align*}
                        \lb f\lb X\rb g\lb X\rb \rb_{i, j}
                        \;=\;
                        \overset{n}{\underset{k=1}{\Sigma}}\, f\lb X\rb_{i k} g\lb X\rb_{k j} 
                    \end{align*}
                    And from the sub additive property (\ref{lem24}) of the $sep-rank$ we get 
                    \begin{align*}
                        & sep-rank\lb \lb f\lb X\rb g\lb X\rb \rb_{i, j}\rb 
                        \;=\;
                        sep-rank\lb \overset{n}{\underset{k=1}{\Sigma}}\, f\lb X\rb_{i k} g\lb X\rb_{k j}\rb 
                        \\ &
                        \;\leq\;
                        \overset{n}{\underset{k=1}{\Sigma}}\, sep-rank\lb f\lb X\rb_{i k} g\lb X\rb_{k j}\rb 
                        \\ &
                        \underbrace{\leq}_\textit{Lemma (\ref{lem212})} 
                        \overset{n}{\underset{k=1}{\Sigma}}\, sep-rank\lc f\lb X\rb_{i k}\rc \cdot sep-rank\lc g\lb X\rb_{k j}\rc 
                        \\ &
                        \;\leq\;
                        n \cdot
                        \underset{i, k}{\max}\; sep-rank\lc f\lb X\rb_{i k}\rc 
                        \cdot
                        \underset{k, j}{\max}\; sep-rank\lc g\lb X\rb_{k j}\rc
                    \end{align*}
                    \begin{align*}
                        & \;=\; 
                        n \cdot sep-rank\lc f\lb X\rb\rc 
                        \cdot sep-rank\lc g\lb X\rb\rc   \quad\blacksquare 
                    \end{align*}    
            \item[(iv)] 
                    Let fix some indices $i\in \lc r\rc$ and $j \in \lc n \rc$ then we have 
                    \begin{align*}
                        &
                        \lb W f\lb X\rb \rb_{i, j} = 
                        \overset{n}{\underset{k=1}{\Sigma}}\;
                        W_{i k}  f\lb X\rb_{k j}
                    \end{align*}
                    Hence 
                    \begin{align*}
                        & 
                        sep-rank\lb \lb W f\lb X\rb \rb_{i, j}\rb 
                        \underbrace{\;\leq\;\quad}_\textit{Lemma (\ref{lem24})}
                        \overset{n}{\underset{k=1}{\Sigma}}\; sep-rank\lb W_{i k} 
                        f\lb X\rb_{k j}\rb 
                        \\ &
                        \quad\quad
                        \;\leq\; 
                        n 
                        \underset{i, j \in \lc n\rc \times \lc m\rc }{\max} sep-rank\lb f\lb X\rb_{i j}\rb
                        \;=\;
                        n \cdot \; sep-rank\lb f\lb X\rb\rb  
                        \quad\;\;\blacksquare
                    \end{align*}
        \end{description}
    \end{adjustwidth}
\end{proof} 


\begin{remark}
    The last two sep-rank upper bounds lemmas (\ref{lem_547}), (\ref{lem_548}) 
    hold for the $\sup-sep$ metric as well, and can be obtained 
    simply by replacing every $sep-rank$ by $\sup-sep$ in the lemma. 
    The proof is also the same up to replacing every 
    $sep-rank$ by $\sup-sep$ in the proof as well.
\end{remark}
