# Supplementary material for: Transformer Vs. MLP-Mixer: Exponential Expressive Gap For NLP Problems
Source: arXiv:2208.08191 source file (2022-11-17)
Supplement: Supplementary file 3 [file appendix_B.tex]

\section{Layer upper-bound lemma}
\subsection{Lemma 5.2}
\begin{lemma}\label{lem55}
    Let $L_{mlp}$, be a general mlp layer, as defined by 
    \equ{
        L_{i,\; m, n}^{2, \,mlp}\lb X\rb = 
        \sigma_2\lb \mathbf{1}_O\lc i\rc \cdot W_i^o \pi_e \lb X\rb  
        + \mathbf{1}_E\lc i\rc \cdot \lc W_i^e \pi_o \lb X^T\rb \rc^T \rb
        + \mathbf{1}_R\lc i\rc \pi_r\lb X\rb 
    } 
    And a function $f: \mathcal{X}^M \to \mathbb{R}^{n \times m}$. 
    Then we have the following upper bound, on the separation-rank. 
    \equ{\label{eq169}
        sep-rank\lc L_{i,\;k, m, n}^{2, \,mlp}\circ f\lb X\rb\rc \leq 
        n^2\,\cdot\, sep-rank\lc f\lb X\rb\rc^2 + sep-rank\lc f\lb X\rb\rc
    }
\end{lemma}

\begin{proof}
    Using the definition of $L_{MM}^{n, m}$ from equation (\ref{eq162}) we get 
    \begin{align}\label{eq177}
        & 
        sep-rank\lc L_{MM}^{k, m, n}\lb f\lb X\rb\rb \rc 
    \end{align}
    \begin{align*}
        &
        \;=\;
        sep-rank\lc 
             \sigma_2\lb 
                \mathbf{1}_E\lc k\rc \cdot \lc W_k^e \pi_e \circ  f\lb X\rb^T\rc^T
                + 
                \mathbf{1}_O\lc k\rc \cdot W_k^o \pi_o \circ f\lb X\rb
            \rb 
            + 
            \mathbf{1}_E\lc k\rc \pi_r \circ f\lb X\rb
        \rc 
    \end{align*}
    \begin{align}\label{eq178}
        & 
        \;=\;
        sep-rank\lc 
             \mathbf{1}_O\lc k\rc \sigma_2\lb  W_k^o \pi_o \circ f\lb X\rb\rb 
             + \mathbf{1}_E\lc k\rc \cdot 
             \sigma_2\lb \lb W_k^e \pi_e \circ f\lb X\rb^T\rb^T \rb
             + \mathbf{1}_E\lc k\rc \pi_r \circ f\lb X\rb
        \rc
    \end{align}
    And let turn into case analysis then \\
    \textbf{Case-1:}
    $\quad k \in O\quad$ using equations (\ref{eq178}) and (\ref{eq177}) we have 
    \begin{align*}
        & 
        sep-rank\lc L_{MM}^{k, m, n}\lb f\lb X\rb\rb \rc 
        \\ & 
        \;=\;
        sep-rank\lc 
             \mathbf{1}_O\lc k\rc 
             \sigma_2\lb  W_k^o \pi_o \circ f\lb X\rb\rb  
             + \mathbf{1}_E\lc k\rc \cdot 
             \sigma_2\lb \lb W_k^e \pi_e \circ f\lb X\rb^T\rb^T \rb
             + \mathbf{1}_E\lc k\rc  \pi_r \circ f\lb X\rb
        \rc
    \end{align*}
    \begin{align*}
        &
        \underbrace{\;=\;}_{k \in O}
        sep-rank\lc 
              \sigma_2\lb  W_k^o  \pi_o \circ f\lb X\rb\rb
              \;+\; 
              \mathbf{1}_E\lc k\rc  \pi_r \circ f\lb X\rb
        \rc
        \\ & 
        \underbrace{\;\leq\;}_\textit{sub-additive} 
            sep-rank\lc \sigma_2\lb  W_k^o  \pi_o \circ f\lb X\rb\rb\rc
        \;+\; 
            sep-rank\lc \mathbf{1}_E\lc k\rc  \pi_r \circ f\lb X\rb\rc
      \\ & 
        \;=\;
        sep-rank\lc \lb W_k^o  \pi_o \circ f\lb X\rb\rb^{\odot 2}\rc
        \;+\; 
        \mathbf{1}_E\lc k\rc  \,\cdot\, sep-rank\lc \pi_r \circ f\lb X\rb\rc
        \\ & 
        \leq 
        sep-rank\lc \lb W_k^o  \pi_o \circ f\lb X\rb\rb^{\odot 2}\rc
        \;+\; 
        sep-rank\lc \pi_r \circ f\lb X\rb\rc
        \\ &
        \underbrace{\;\leq\;}_\textit{Lemma (\ref{lem22})}
        sep-rank\lc \lb W_k^o  \pi_o \circ f\lb X\rb\rb\rc^{2}
        \;+\; 
        sep-rank\lc \pi_r \circ f\lb X\rb\rc
        \\ & 
        \underbrace{\;\leq\;}_\textit{Lemma (\ref{lem21})}
        \lb \dim_{col}\lb W_k^o\rb\cdot sep-rank\lc \pi_o \circ f\lb X\rb \rc \rb^{2}
        \;+\; 
        sep-rank\lc \pi_r \circ f\lb X\rb\rc
        \\ & 
        \;=\;
        n^2 \cdot sep-rank\lc \pi_o \circ f\lb X\rb \rc^2
        \;+\; 
        sep-rank\lc \pi_r \circ f\lb X\rb\rc
        \\ & 
        \underbrace{\;=\;}_\textit{Lemma (\ref{permu_lemma})}
        n^2 \cdot sep-rank\lc f\lb X\rb \rc^2
        \;+\;
        sep-rank\lc f\lb X\rb\rc 
    \end{align*}
    \textbf{Case-2:} 
    $\quad k\in E\quad$ using equations (\ref{eq178}) and (\ref{eq177}) we have 
    \begin{align*}
        & sep-rank\lc L_{MM}^{k, m, n}\lb f\lb X\rb\rb \rc 
        \\ & 
        \;=\;
        sep-rank\lc 
             \mathbf{1}_O\lc k\rc   \cdot \sigma_2\lb  W_k^o \pi_o \circ f\lb X\rb\rb
             + \mathbf{1}_E\lc k\rc \cdot \sigma_2\lb \lb W_k^e \pi_e\lb f\lb X\rb\rb^T\rb^T \rb
             + \mathbf{1}_E\lc k\rc  \pi_r \circ f\lb X\rb
        \rc
        \\ & 
            \underbrace{\;=\;}_{k \in E}
            sep-rank\lc 
                 \sigma_2\lb \lb W_k^e  \pi_e\lb f\lb X\rb\rb^T\rb^T \rb
                 +  \pi_r \circ f\lb X\rb
            \rc
        \\ & 
            \underbrace{\leq}_\textit{Lemma (\ref{lem24})} 
            sep-rank\lc \sigma_2\lb \lb W_k^e \pi_e\lb f\lb X\rb\rb^T\rb^T\rb\rc
            + 
            sep-rank\lc \pi_r \circ f\lb X\rb \rc
        \\ & 
            \;=\;
            sep-rank\lc \lb \lb W_k^e  \pi_e\lb f\lb X\rb\rb^T\rb^T\rb^{\odot 2}\rc
            +
            sep-rank\lc \pi_r \circ f\lb X\rb \rc 
        \\ &
            \underbrace{\;\leq\;}_\textit{Lemma (\ref{lem22})}
            sep-rank\lc \lb W_k^e \pi_e\lb f\lb X\rb\rb^T\rb^T\rc^{2}
            + sep-rank\lc \pi_r \circ f\lb X\rb \rc
        \\ &
            \underbrace{\;=\;}_\textit{Lemma (\ref{lem225})}
            sep-rank\lc W_k^e \pi_e\lb f\lb X\rb\rb^T\rc^{2}
            + sep-rank\lc \pi_r \circ f\lb X\rb \rc
    \end{align*}
    \begin{align*} 
        &
             \underbrace{\;\leq\;}_\textit{Lemma (\ref{lem21})}
            \lb \dim_{col}\lb W_k^e\rb\cdot sep-rank\lc  \pi_e\lb f\lb X\rb\rb^T \rc \rb^{2}
            + sep-rank\lc \pi_r \circ f\lb X\rb \rc
            \quad\quad\quad\quad\quad\quad
    \end{align*}
    \begin{align*} 
        & 
            \underbrace{\;=\;}_\textit{Lemma (\ref{lem225})}
            \lb \dim_{col}\lb W_k^e\rb\cdot sep-rank\lc \pi_e\lb f\lb X\rb\rb \rc \rb^{2}
            + sep-rank\lc \pi_r \circ f\lb X\rb \rc  
            \quad\quad\quad\quad\quad\quad
        \\ & 
             \;=\;
            n^2 \cdot sep-rank\lc \pi_e\lb f\lb X\rb\rb \rc^2
            + sep-rank\lc \pi_r \circ f\lb X\rb \rc 
        \\ & 
            \underbrace{\;=\;}_\textit{Lemma (\ref{permu_lemma})}
            n^2 \cdot sep-rank\lc f\lb X\rb \rc^2
            + sep-rank\lc f\lb X\rb \rc
            \QED        
    \end{align*}
\end{proof}
