# Supplementary material for: Transformer Vs. MLP-Mixer: Exponential Expressive Gap For NLP Problems
Source: arXiv:2208.08191 source file (2022-11-17)
Supplement: Supplementary file 4 [file appendix_C.tex]

\section{Mixer bound}
\subsection{Theorem 5.3}
\begin{theorem}\label{thm57}
    Let 
    $\;y_{p,\; m,n}^{2, \, mlp}\;: \mathbb{R}^{n \times m} \to \mathbb{R}^{n \times m}$ be an mlp-based architecture. With depth $p$, 
    of the form 
    $y_{p,\; m,n}^{2,\, mlp}\lb X\rb \,=\, 
    L_{p,\; m, n}^{2, \,mlp}
    \circ \;.\,.\,.\;\circ 
    L_{1,\; m, n}^{2, \,mlp}
    \lb X\rb
    $
    Then we have, the following bound on the separation-rank, of the entire model, 
    \equ{
        sep-rank\lb \,y_{p,\; m,n}^{2, \,mlp}\,\rb 
        \;\leq\; 
        \lb 2 H \cdot m^2 \,\cdot \, n^2\rb^{2^p}
    }
    Writing differently, we have 
    \equ{
        \ln\lb\, sep-rank\lc \,y_{p,\; m,n}^{2, \, mlp}\,\rc \,\rb 
        \;\leq\; 
        \ln \lb\, 2 H \cdot m^2 \,\cdot \, n^2 \;\rb \, \cdot\, 2^p
    }
\end{theorem}

\begin{proof}
    Let 
    $y = y_{MM}^{p,m, n}$
    then $y$ can be written as composition of $p$ layers
    \begin{align*}
        y = L_p \circ ... \circ L_1\lb X\rb
    \end{align*}
    and by the last lemma (\ref{lem55}), each of the layers $L_i$ satisfies 
    \begin{align*}
        sep-rank\lb L_{i}^{n, m} \circ f\lb X\rb\rb \;\leq\; n^2 \cdot sep-rank\lc f\lb X\rb \rc^2 + sep-rank\lc f\lb X\rb \rc        
    \end{align*}    
    denoting
    \begin{align*}
        f\lb p\rb \;\equiv\; sep-rank\lc y_p\rc = sep-rank\lc L_p \circ ... \circ L_1\lb X\rb\rc        
    \end{align*}
    and using lemma (\ref{lem55}) we get the following recursion formula 
    \begin{align*}
        & 
        f\lb p\rb 
        \defeq  sep-rank\lc L_p \circ ... \circ L_1\lb X\rb\rc
        \\ & 
        \;=\;   sep-rank\lc L_p \circ L_{p-1}\circ  ... \circ L_1\lb X\rb\rc
        \;=\;   sep-rank\lc L_p \circ y_{p-1}\lb X\rb\rc
        \\ & 
        \underbrace{\leq}_\textit{Lemma (\ref{lem55})}
        n^2 \cdot sep-rank\lc y_{p-1}\lb X\rb\rc^2
        \;+\; 
        sep-rank\lc y_{p-1}\lb X\rb\rc
        \\ & 
        \underbrace{\leq}_{sep-rank\lc y_{p-1}\lb X\rb\rc \geq 1}
        \lb n^2 +1\rb\cdot \lb sep-rank\lc y_{p-1}\lb X\rb\rc\rb^2
        \;=\; \lb n^2+1\rb f\lb p-1\rb^2        
    \end{align*}
    So we end with the following recursion formula  
    \equ{\label{eq199}
        f\lb p\rb \;\leq\; \lb n^2+1\rb f\lb p-1\rb^2
    }
    Moving for the base case $p=1$ we have 
    \begin{align*}
        & 
        f\lb 1\rb = sep-rank\lc L_1\circ Id\lb X\rb\rc
        \\ & 
        \underbrace{\leq}_\textit{Lemma (\ref{lem55})}
        n^2 \cdot sep-rank\lc Id\lb X\rb\rc^2 + sep-rank\lc Id\lb X\rb\rc        
        \\ & 
        \underbrace{\leq}_\textit{Lemma (\ref{lem218})}
        n^2 \cdot 2^2 + 2 = 4 \cdot n^2 + 2
    \end{align*}
    Altogether we get the following recursion formula 
    \equ{\label{eq202}
        f\lb p\rb \;\leq\; \lb n^2+1\rb f\lb p-1\rb^2
        \quad\quad\bigwedge\quad\quad
        f\lb 1\rb \leq 4 \cdot n^2 + 2
    }
    And by easy induction
    \begin{align*}
        &
        f\lb p\rb \;\leq\; \lb n^2+1\rb f\lb p-1\rb^2 
        \;\leq\; \lb n^2+1\rb  \lb\lb n^2+1\rb f\lb p-2\rb^2\rb^2
        \\ & 
        \;=\; \lb n^2+1\rb \lb n^2+1\rb^2 f\lb p-2\rb^{2^2}
        \;\leq\; \lb n^2+1\rb \lb n^2+1\rb^2 \lb n^2+1\rb^{2^2} f\lb p-3\rb^{2^3}
        \\ & 
        \underbrace{\leq\; .\,.\,.\;\leq}_\textit{easy induction}
        \lb n^2+1\rb \lb n^2+1\rb^2 \lb n^2+1\rb^{2^2} \cdot \,.\,.\,.\,\cdot\lb n^2+1\rb^{2^2} \lb n^2+1\rb^{2^{p-2}} \cdot f\lb 1\rb^{2^{p-1}}
        \\ & 
        \underbrace{\leq}_\textit{Equation (\ref{eq202})} 
        \lb \overset{p-2}{\underset{k=0}{\prod}}\; \lb n^2+1\rb^{2^k}\rb
        \cdot
        \lb 4 n^2 + 2\rb^{2^{p-1}} 
        \leq 
        4^{2^{p-1}} \cdot \overset{p-1}{\underset{k=0}{\prod}}\; \lb n^2+1\rb^{2^k}
        \\ & 
        =
        4^{2^{p-1}} \cdot \lb n^2+1\rb^{\overset{p-1}{\underset{k=0}{\Sigma}}\; 2^k}
        =
        2^{2^p} \lb n^2+1\rb^{2^p-1} 
        \leq 
        2^{2^p} \lb n^2+1\rb^{2^p}
        \\ & 
        =
        \lb 2 n^2+2\rb^{2^p}
        \leq 
        \lb 2 n^2 + H m^2\rb^{2^p}
        \leq 
        \lb 2 H m^2 n^2\rb^{2^p}
        \QED 
    \end{align*}
\end{proof}
