# Supplementary material for: Transformer Vs. MLP-Mixer: Exponential Expressive Gap For NLP Problems
Source: arXiv:2208.08191 source file (2022-11-17)
Supplement: Supplementary file 5 [file appendix_D.tex]

\section{Transformer Bound}
\subsection{Theorem 5.4}
\begin{theorem}\label{thm220}\label{229}
    Let 
    $y_{p, H}^{R}:
    M_{n \times m}\lb \mathbb{R}\rb 
    \to M_{n \times m}\lb \mathbb{R}\rb$, 
    be transformer architecture. 
    Without activations, and normalization layers,
    with depth $p$ and residual connections, of the form 
    \equ{
        y_{p, H}^{R}\lb X\rb = L_{p, H}^{R} \circ ... \circ L_{1, H}^{R}\lb X\rb 
    }
    With all the layers, and matrices, have the same dimensions, $W_p^{i j} \in M_{m \times n}\lb \mathbb{R}\rb$. 
    Then, the following bound, on the separation rank holds
    \equ{\label{eq730}
        sep-rank\lb y_{p, H}^{R}\rb
        \;\leq\;
        \lb 2 H \cdot m^2 \,\cdot \, n^2\rb^{3^p}
    }    
\end{theorem}


\subsection{Proof}
\subsubsection{Simpler theorem}
We will start by proving the following simpler claim.
For transformer like architecture but without residual 
connections and transposes.
\begin{theorem}\label{thm220}\label{229}
    Let 
    $y_{p, H}^{R}:
    M_{n \times m}\lb \mathbb{R}\rb 
    \to M_{n \times m}\lb \mathbb{R}\rb$, 
    be transformer architecture. 
    Without activations, and normalization layers, 
    residual connections, or transposes.
    With depth $p$, of the form 
    \equ{
        y_{p}\lb X\rb = L_{p} \circ ... \circ L_{1}\lb X\rb 
    }
    And each layer $L_i$ is of the form 
    \equ{
        L_i\lb X\rb \;=\; \overset{3}{\underset{i=1}{\prod}}\; W_i X
    }
    With all the layers, and matrices, have the same dimensions, 
    $W_p^{i j} \in M_{m \times n}\lb \mathbb{R}\rb$. 
    Then, the following bound, on the separation rank holds
    \equ{\label{eq730}
        sep-rank\lb y_{p, H}^{R}\rb
        \;\leq\;
        \lb 2 H \cdot m^2 \,\cdot \, n^2\rb^{3^p}
    }    
\end{theorem}

\begin{proof}
    For mathematical convenience we will prove 
    the following more general claim, that for every
    function obtained by layers
    composition of the form, 
    $y_{p, H}^{R, d} = 
    L_p^d \circ ... \circ L_1^d\lb X\rb$.
    Where $L_i^d\lb X\rb$ is the $i$ layer. And is of the form, 
    \equ{
        L_i^d\lb X\rb = \overset{d}{\underset{i=1}{\prod}}\; W_i X
    }
    We have that 
    \equ{
        sep-rank\lb y_{p, H}^{R, d}\rb
        \;\leq\;
        \lb 2 H \cdot m^2 \,\cdot \, n^2\rb^{d^p}
    }
    The claim of the statement will follow 
    as particular case for $d=3$.
    We will start by proving for small $p$'s since 
    those are the simpler cases, and then we will 
    show by induction, that the claim is true for every $p\in \mathbb{N}$.\\
    \textbf{Case-1:}  $p=1$ in this case $y_p = L_1 \circ Id \lb X\rb$ and by Lemma (\ref{lem216}) we have 
    \begin{align*}
        & 
        sep-rank\lc y_p\rc 
        \,=\,
        sep-rank\lc L_1^d \circ Id \lb X\rb\rc 
        \\ & 
        \underbrace{\leq}_\textit{Lemma (\ref{lem216})}
        m^{d-1} \cdot n^d  \cdot \lc sep-rank\lb I\lb X\rb\rb\rc^d 
        \underbrace{\leq}_{Lemma (\ref{lem218})}  2^d \cdot n^d \cdot m^{d-1}
    \end{align*}
    \textbf{Case-2:} $p=2$ in this case we have
    \begin{align*}
        & 
        sep-rank\lc y_p^d\rc 
        \;=\; 
        sep-rank\lc L_2^d  \circ L_1^d\lb X\rb\rc
        \underbrace{\;\leq\;}_\textit{Lemma (\ref{lem216})}
        m^{d-1}\cdot n^d\cdot \lb sep-rank\lc L_1^d\lb X\rb\rc\rb^d 
        \\ &
        \underbrace{\;\leq\;}_\textbf{Case-1} 
        m^{d-1}\cdot n^d\cdot \lb 2^d n^d m^{d-1}\rb^d 
        \;=\;
        \lc m^{d-1} \cdot n^d\rc \cdot \lc 2^{d^2} n^{d^2} m^{d\lb d-1\rb} \rc 
        \;=\;
        2^{d^2} n^{d^2 + d} m^{\lb d+1\rb \lb d-1\rb }  
    \end{align*}
    \textbf{Case-3:} For general $p \in \mathbb{N}$ with $p \geq 2$ we have 
    \begin{align*}
        & 
        sep-rank\lc y_p^d\rc 
        \;=\; 
        sep-rank\lc L_p^d  \circ ...  \circ L_1^d\lb X\rb\rc
        \\ & 
        \underbrace{\;\leq\;}_\textit{Lemma (\ref{lem216})}
        m^{d-1}\cdot n^d\cdot \lb sep-rank\lc L_{p-1}^d  \circ ...  \circ L_1^d\lb X\rb\rc\rb^d
    \end{align*}
    Denoting
    \begin{align*}
        f\lb p, d\rb \equiv sep-rank\lc y_p^d\rc
    \end{align*}
    we have the following two rules
    \begin{align*}
        & 
        \textit{(1)}\quad\quad  f\lb p, d\rb \;\leq\; m^{d-1} \cdot n^d \cdot f\lb p-1, d\rb^d
        \\ & 
        \textit{(2)}\quad\quad f\lb 1, d\rb \;\leq\; 2^d \cdot n^d \cdot m^{d-1}        
    \end{align*}
    Hence 
    \begin{align*}
        & 
        f\lb p, d\rb \;\leq\; m^{d-1} \cdot n^d \cdot f\lb p-1, d\rb^d
        \;\leq\; m^{d-1} \cdot n^d \cdot  \lc m^{d-1}\cdot n^d\cdot f\lb p-2, d\rb^d\rc^d 
        \\ &
        \;=\; \underbrace{\lc m^{d-1} \cdot n^d\rc }_{\Delta} \cdot  \underbrace{\lc m^{d-1}\cdot n^d\rc^d}_{\Delta^d} \cdot f\lb p-2, d\rb^{d^2}
        \;=\; \Delta \cdot \Delta^d \cdot f\lb p-2, d\rb^{d^2}
        \\ & 
        \;\leq\; \Delta \cdot \Delta^d \cdot \Delta^{d^2} \cdot f\lb p-3, d\rb^{d^3} 
        \underbrace{\;\leq\; .\,.\,. \;\leq\;}_\textit{$k-3$ more steps} 
        \lc \overset{k-1}{\underset{i=0}{\prod}}\, \Delta^{d^i} \rc \cdot f\lb p-k, d\rb^{d^k}
        \\ & 
        \underbrace{\;\leq\; .\,.\,. \;\leq\;}_\textit{after $n-1$ steps} 
        \lc \overset{p-2}{\underset{i=0}{\prod}}\, \Delta^{d^i} \rc \cdot f\lb 1, d\rb^{d^{n-1}}
        \;=\; 
        \lc \overset{p-2}{\underset{i=0}{\prod}}\, \Delta^{d^i} \rc \cdot \lc 2^d \Delta\rc^{d^{p-1}}
        \\ & 
        \;=\; 
        2^{d^n} \, \overset{p-1}{\underset{i=0}{\prod}}\, \Delta^{d^i} 
        \;=\; 
        2^{d^n} \, \Delta^{\overset{p-1}{\underset{i=0}{\Sigma}}\, d^i}
        \;=\;
        2^{d^p} \, \Delta^{\frac{d^p-1}{d-1}}
        \;=\; 
        2^{d^p} \, \lc m^{d-1} n^d\rc^{\frac{d^p-1}{d-1}}
        \\ &
        \;=\; 
        2^{d^p} \, \cdot\, m^{d^p-1} \cdot n^{d \frac{d^p-1}{d-1}}
        \;\leq\; 
        2^{d^p} \, \cdot\, m^{d^p} \cdot n^{2 d^p}
        \;=\; 
        \lb 2 \cdot m \cdot n^2 \rb^{d^p}\QED 
    \end{align*}
\end{proof}

\begin{lemma}
    \label{lem216}
    Let $L^d$ be polynomial transformer layer of degree $d$ of the form
    \equ{
        L^d \lb X\rb \defeq W_d \cdot  X \cdot W_{d-1} X \cdot ... \cdot W_1 X 
    }
    And let $f:\mathcal{X}^{2 M} \to \mathbb{R}^{n \times m}$ be some function with separation rank $k_f$ then for  
    \equ{
        \lc L^d \circ f\rc \lb X\rb = W_d \cdot f\lb X\rb\cdot W_{d-1}\cdot f\lb X\rb \cdot ... \cdot W_1\cdot f\lb X\rb 
    }
    We have
    \equ{
        sep-rank\lb L^d \circ f\rb \leq m^{d-1} \cdot n^{d} \cdot \lb sep-rank\lc f\lb X\rb\rc \rb^{d}
    }
\end{lemma}

\begin{proof}
        We will prove by induction on $d$ \\
    \textbf{Case-1:} $d=1$ then we would have $L^d\lb X\rb = W_1 f\lb X\rb$ and by (\ref{lem21}) we get
    \equ{
        sep-rank\lc W_1 f\lb X\rb \rc \;\leq\; n \cdot sep-rank\lc f\lb X\rb\rc 
    }
    \textbf{Case-2:} $d=2$ so 
    \equ{
        L^2\circ f\lb X\rb \,=\, W_1 \cdot f\lb X\rb \cdot W_2 \cdot f\lb X\rb 
    }
    Hence
    \begin{align*}
        & \quad
        sep-rank\lc L^2\circ f\lb X\rb\rc
        \;=\; sep-rank\lc W_1 \cdot f\lb X\rb \cdot W_2 \cdot f\lb X\rb \rc 
    \end{align*}
    \begin{align*}
        &
        \underbrace{\;\leq\;}_\textit{Lemma (\ref{lem214})} 
        m \,\cdot\, sep-rank\lc W_1 \cdot f\lb X\rb \rc \,\cdot\, sep-rank\lc W_2 \cdot f\lb X\rb \rc  
        \\& 
        \underbrace{\;\leq\;}_\textit{Lemma (\ref{lem21})} m \cdot n^2 \cdot \lb sep-rank\lc f\lb X\rb\rc \rb^2 
    \end{align*}
    \textbf{Case-3:} For general $d \in \mathbb{N}$ with $d \geq 2$ then assume by induction that for $d-1$ we have 
    \equ{\label{eq48}
        sep-rank\lc L^{d-1}\circ f\lb X\rb\rc \leq m^{d-2} \cdot n^{d-1} \cdot \lb sep-rank\lc f\lb X\rb\rc \rb^{d-1}
    }
    Then for $d$ we have
    \begin{align*}
        & sep-rank\lc L^d\circ f\lb X\rb\rc = sep-rank \lc W_d f\lb X\rb L^{d-1}\circ f\lb X\rb \rc 
        \\ & 
        \underbrace{\leq}_\textit{Lemma (\ref{lem214})} 
        m \,\cdot\, sep-rank\lc W_1 \cdot f\lb X\rb \rc \,\cdot\, sep-rank\lc L^{d-1} \circ f\lb X\rb \rc
        \\ & 
        \underbrace{\;\leq\;}_\textit{Lemma (\ref{lem21})} m \cdot n \cdot sep-rank\lc f\lb X\rb\rc \, \cdot\, sep-rank\lc L^{d-1} \circ f\lb X\rb \rc 
        \\ & 
        \underbrace{\leq}_\textit{Induction Hypothesis (\ref{eq48})} 
        m^{d-1} \cdot n^{d} \cdot \lb sep-rank\lc f\lb X\rb\rc \rb^{d}\quad\quad \blacksquare 
    \end{align*}
\end{proof}

\begin{remark}
    The last theorem implies in particular that for $y_p^d$ be degree $d$ linear transformer then 
    \equ{
        \epsilon-sep-rank\lb y_p^d\rb \;\leq\; \lb 2 \cdot m \cdot n^2\rb^{d^p}
    }       
\end{remark}

\begin{proof}
    Using the $\epsilon-rank$ definition we have 
    \begin{align*}
        & 
        \epsilon-sep-rank\lb y_p^d\rb
        \;=\;
        \underset{f \in \mathbb{B}_\epsilon^{\norm{.}_\infty}\lb y_p^d\rb}{\min}\; sep-rank\lb f\rb
        \\ & 
        \underbrace{\;\leq\;}_{y_p^d \in \mathbb{B}_\epsilon^{\norm{.}_\infty}\lb y_p^d\rb} 
        sep-rank\lb y_p^d\rb  
        \underbrace{\;\leq\;}_\textit{Theorem \ref{thm220}}
        \lb 2 \cdot m \cdot n^2\rb^{d^p} \quad\blacksquare        
    \end{align*}
\end{proof}

\subsubsection{ 
    Generalizing to multi-head with 
    residual connections and transposes
}

\begin{definition}
    \label{def224}
    Let $y_{p, H}$ be linear transformer architecture with multi-head attention and residual connections of the form
    \equ{
        y_{p, H}\lb X\rb 
        \,\defeq\,
        L_{p, H}^{R} \circ ... \circ L_{1, H}^{R}\lb X\rb 
    }
    Where each $L_{i,\, H}^{R}:\mathcal{X}^N \to \mathcal{X}^M$ is of the form 
    \equ{
        L_{i, H}^{R}\lb X\rb 
        \,=\, 
        W_O \cdot \lb 
        \overset{H}{\underset{k=1}{\Sigma}}\;\,
        \overset{3}{\underset{j=1}{\prod}}\; 
        \lb 
            \mathbf{1}_{T_k}\lc j\rc \cdot \lb W^{j, k} X\rb 
            \,+\, 
            \mathbf{1}_{T_k^c}\lc j\rc \cdot \lb W^{j, k} X\rb^T
        \rb\rb + \mathbf{1}_R\lc i\rc\, X
    }
    Where
    \equ{
        \forall k \quad T_k \subset \lc \,3\,\rc  
    } 
    Is the subset of indices where transpose should be taken.
\end{definition}

\begin{theorem}\label{229}
    Let $y_{p, H}^{R}: M_{n \times m}\lb \mathbb{R}\rb \to M_{n \times m}\lb \mathbb{R}\rb$
    be linear transformer with depth $p$ residual connections, and transposes of the form 
    \equ{
        y_{p, H}^{R}\lb X\rb = L_{p, H}^{R} 
        \circ ... \circ 
        L_{1, H}^{R}\lb X\rb 
    }
    With all the layers and matrices have the same dimensions, $W_p^{i j} \in M_{m \times n}\lb \mathbb{R}\rb$ 
    then the following bound on the separation rank holds
    \equ{\label{eq730}
        sep-rank\lb y_{p, H}^{R, d}\rb
        \;\leq\;
        \lb 2 H \cdot m^2 \,\cdot \, n^2\rb^{3^p}
    }
\end{theorem}

\begin{proof}
    For mathematical convenience we will prove 
    the following more general claim, that for every
    function obtained by layers
    composition of the form, 
    $y_{p, H}^{R, d} = 
    L_{p, H}^{R, d} \circ ... \circ L_{1, H}^{R, d}\lb X\rb$.
    Where $L_{p, H}^{R, d}\lb X\rb$ is the $i$ layer. And is of the form, 
     \equ{
        L_{i, H}^{R, d}\lb X\rb 
        \,=\, 
        W_O \cdot \lb 
        \overset{H}{\underset{k=1}{\Sigma}}\;\,
        \overset{d}{\underset{j=1}{\prod}}\; 
        \lb 
            \mathbf{1}_{T_k}\lc j\rc \cdot \lb W^{j, k} X\rb 
            \,+\, 
            \mathbf{1}_{T_k^c}\lc j\rc \cdot \lb W^{j, k} X\rb^T
        \rb\rb + \mathbf{1}_R\lc i\rc\, X
    }
    We have that 
    \equ{
        sep-rank\lb y_{p, H}^{R, d}\rb
        \;\leq\;
        \lb 2 H \cdot m^2 \,\cdot \, n^2\rb^{d^p}
    }
    The claim of the statement will follow as particular case for $d=3$. \\
    Using the second promise (\ref{660}) of the previous Lemma (\ref{lem227}) we know
    \equ{\label{eq740}
        sep-rank\lb L_{H}^{R, d}\circ f\lb X\rb\rb 
        \leq 
        H \cdot m^{d} \,\cdot \, n^{d+1} \cdot \, \lb sep-rank\lc f\lb X\rb \rc\,\rb^d
    }
    While we are interested at finding
    \begin{align*}
        sep-rank\lb y_{p, H}^{R, d}\lb X\rb\rb
         = 
        sep-rank\lb L_{p, H}^{R, d} \circ ... \circ L_{1, H}^{R, d}\lb X\rb \rb      
    \end{align*}
    denoting 
    \begin{align*}
        f\lb p\rb \defeq sep-rank\lb L_{p, H}^{R, d} \circ ... \circ L_{1, H}^{R, d}\lb X\rb \rb        
    \end{align*}
    equation (\ref{eq740}) gives us, 
    \begin{align*}
        & 
            f\lb p\rb
             = 
            sep-rank\lb L_{p, H}^{R, d} \circ ... \circ L_{1, H}^{R, d}\lb X\rb \rb
        \\ & 
             = 
            sep-rank\lb L_{p, H}^{R, d} \lb  L_{p-1, H}^{R, d}\circ ... \circ L_{1, H}^{R, d}\lb X\rb \rb \rb
        \\ & 
        \underbrace{\leq\;\;\;}_\textit{Equation (\ref{eq740})}
        H \cdot m^{d} \,\cdot \, n^{d+1} \cdot \,
        \lb sep-rank\lc L_{p-1, H}^{R, d}\circ ... \circ L_{1, H}^{R, d}\lb X\rb \rc\rb^d
        \\ & 
        \eqdef\;
        H \cdot m^{d} \,\cdot \, n^{d+1} \cdot \,\lb f\lb p-1\rb\rb^d
    \end{align*}
    hence we have 
    \equ{\label{eq790}
        f\lb p\rb \leq H \cdot m^{d} \,\cdot \, n^{d+1} \cdot \,\lb f\lb p-1\rb\rb^d
    }
    denoting 
    \equ{\label{eq800}
        \Delta \equiv H \cdot m^{d} \,\cdot \, n^{d+1}
    }
    equation (\ref{eq790}) becomes 
    \begin{align*}
        f\lb p\rb \;\leq\; \Delta \cdot \,\lb f\lb p-1\rb\rb^d
    \end{align*}
    to conclude this argument using easy induction we get
    \begin{align*}
        &
        f\lb p\rb \;\leq\; \Delta \cdot \,\lb f\lb p-1\rb\rb^d
        \;\leq\; \Delta \cdot \Delta^d \cdot \lb f\lb p-2\rb\rb^{d^2}
        \\ &
        \leq\; \Delta \cdot \Delta^d \cdot \Delta^{d^2} \cdot \lb f\lb p-2\rb\rb^{d^3}
        \leq \;.\;.\;.\; \leq\; 
        \overset{p-2}{\underset{k=0}{\prod}} \Delta^{d^k} \cdot \lb f\lb p-\lb p-1\rb\rb\rb^{p-1}
        \\ & 
        \;=\;
        \overset{p-2}{\underset{k=0}{\prod}} \Delta^{d^k} \cdot \lb f\lb 1\rb\rb^{p-1}
        \;=\;
        \overset{p-2}{\underset{k=0}{\prod}} \Delta^{d^k} \cdot 
        \lb 
            sep-rank\lc L_{1, H}^{R, d} \circ Id \lb X\rb\rc 
        \rb^{p-1}        
        \\ & 
        \underbrace{\,\leq\,}_\textit{Lemma (\ref{lem227})} 
        \overset{p-2}{\underset{k=0}{\prod}} \Delta^{d^k} \cdot \Delta^{p-1} 
        \lb 
            sep-rank\lc Id \lb X\rb\rc 
        \rb^{d^p}
        \\ & 
        \underbrace{\leq}_\textit{Lemma \ref{lem218}}
        2^{d^p} \cdot \overset{p-1}{\underset{k=0}{\prod}}\, \Delta^{d^k} 
        \;=\; 
        2^{d^p} \cdot \Delta^{\overset{p-1}{\underset{k=0}{\Sigma}}\, d^k}
        \\ & 
        \;=\; 
        2^{d^p} \cdot \Delta^{\frac{d^p - 1}{d - 1}}
        \underbrace{\;=\;}_\textit{Equation (\ref{eq800})} 
        2^{d^p} \, \lb H \cdot m^{d} \,\cdot \, n^{d+1}\rb^{\frac{d^p - 1}{d - 1}}
        \\ & 
        \;\leq\;  \lb 2 H \cdot m^{\frac{d}{d-1}} \,\cdot \, n^\frac{d+1}{d-1}\rb^{d^p}
        \;\leq\; \lb 2 H \cdot m^2 \,\cdot \, n^2\rb^{d^p}
    \end{align*}
\end{proof}



\begin{lemma}\label{lem227}
    Let 
    $L_{H}^{R, d}: \mathbb{R}^{n \times m} \to \mathbb{R}^{n \times m}$
    be linear transformer layer,
    \equ{
        L_{i, H}^{R, d}\lb X\rb 
        \,=\, 
        W_O \cdot \lb 
        \overset{H}{\underset{k=1}{\Sigma}}\;\,
        \overset{d}{\underset{j=1}{\prod}}\; 
        \lb 
            \mathbf{1}_{T_k}\lc j\rc \cdot \lb W^{j, k} X\rb  \,+\, \mathbf{1}_{T_k^c}\lc j\rc \cdot \lb W^{j, k} X\rb^T
        \rb\rb + \mathbf{1}_R\lc i\rc\, X
    }
    as in definition (\ref{def224}), 
    And let $f:\mathcal{X}^{2 M} \to \mathbb{R}^{n \times m}$ be a function with separation rank $k_f$ then the following bound on the separation-rank holds
    \equ{\label{eq63}
        sep-rank\lb L_{H}^{R, d}\circ f\lb X\rb\rb 
        \;\leq\;
        \dim_\textit{col}\lb W_O\rb \cdot
        \overset{H}{\underset{k=1}{\Sigma}}\;\,
        \Delta_k
        \;+\; sep-rank\lb f\lb X\rb\rb
    }
    Where
    \begin{equation*}\label{eq640}
        \begin{split}
            &
                \Delta_k 
                \;\equiv\;
                \lb \,\underset{j\in T_k \backslash \ls 1\rs}{\prod}\; \dim_\textit{row}\lb W_{j, k}\rb \rb 
                \,\cdot \,
                \lb \,\overset{d}{\underset{j=1}{\prod}}\; \dim_\textit{col}\lb W^{j, k}\rb \,\rb  
            \\ & 
            \quad\quad\quad
                \cdot
                \lb \dim_\textit{col}\lb f\lb X\rb\rb\rb^{\abs{T_k^c \backslash \ls 1\rs}}
                \, \cdot \, 
                \lb sep-rank\lb f\lb X\rb \rb\,\rb^d   
        \end{split}
    \end{equation*}
    If in addition all the parameters matrices are from the same dimensions i.e 
    \equ{\label{650}
        \forall j, k \quad W_{j, k} \in M_{m \times n}\lb \mathbb{R}\rb
    }
    Then the following simpler upper bound on the separation rank holds
    \equ{\label{660}
        sep-rank\lb L_{H}^{R, d}\circ f\lb X\rb\rb 
        \leq 
        H \cdot m^{d} \,\cdot \, n^{d+1} \cdot \, \lb sep-rank\lc f\lb X\rb \rc\,\rb^d
    }
\end{lemma}

\begin{proof}
        Using $L_H^{R, d}$ definition we get
    \begin{align*}
        & sep-rank\lb L_{H}^{R, d}\circ f\lb X\rb\rb 
        \\ & 
        \underbrace{\,=\,}_\textit{Definition (\ref{def224})} 
        sep-rank\lb W_O \cdot \lb 
        \overset{H}{\underset{k=1}{\Sigma}}\;\,
        \overset{d}{\underset{j=1}{\prod}}\; \lb 
            \mathbf{1}_{T_k}\lc j\rc \cdot \lb W^{j, k} f\lb X\rb\rb  \,+\, \mathbf{1}_{T_k^c}\lc j\rc \cdot \lb W^{j, k} f\lb X\rb\rb^T
        \rb\rb + f\lb X\rb
        \rb 
    \end{align*}
    \begin{align*}
        &
        \underbrace{\leq}_\textit{Lemma (\ref{lem24})} 
        \overset{H}{\underset{k=1}{\Sigma}}\;\,
        sep-rank\lb \lb 
        W_O \cdot \overset{d}{\underset{j=1}{\prod}}\; \lb 
            \mathbf{1}_{T_k}\lc j\rc \cdot \lb W^{j, k} f\lb X\rb\rb  \,+\, \mathbf{1}_{T_k^c}\lc j\rc \cdot \lb W^{j, k} X\rb^T
        \rb\rb
        \rb  
        + sep-rank\lb f\lb X\rb\rb 
     \end{align*}
     \begin{align*}
        & 
        \underbrace{\leq}_{Lemma (\ref{lem214})} 
        \overset{H}{\underset{k=1}{\Sigma}}\;\,
        \dim_\textit{col}\lb W_O\rb \cdot
        sep-rank\lb 
        \overset{d}{\underset{j=1}{\prod}}\; 
        \lb 
            \mathbf{1}_{T_k}\lc j\rc \cdot \lb W^{j, k} X\rb  \,+\, \mathbf{1}_{T_k^c}\lc j\rc \cdot \lb W^{j, k} X\rb^T
        \rb\rb
       + sep-rank\lb f\lb X\rb\rb
    \end{align*}
    \begin{align*}
     & 
        \underbrace{\leq}_{Lemma (\ref{lem218})} 
        \dim_\textit{col}\lb W_O\rb \cdot
        \overset{H}{\underset{k=1}{\Sigma}}\;\,
        \underbrace{
            sep-rank\lb 
            \overset{d}{\underset{j=1}{\prod}}\; W^{j, k} \, \cdot\, 
            \lc 
                \mathbf{1}\lc j\in T_k\rc f\lb X\rb + \mathbf{1}\lc j\in T_k^c\rc f\lb X\rb^T
            \rc\rb
        }_{\Delta_k}
        \;+\; sep-rank\lb f\lb X\rb\rb
    \end{align*}
    \begin{align*}
        & \;\equiv\;
        \dim_\textit{col}\lb W_O\rb \cdot
        \overset{H}{\underset{k=1}{\Sigma}}\;\,
        \Delta_k
        \;+\; sep-rank\lb f\lb X\rb\rb
     \end{align*}
     So it left to bound $\Delta_k$ and indeed
     \begin{align*}
        & \Delta_k 
         \;\defeq\;
         sep-rank\lb 
           \overset{d}{\underset{j=1}{\prod}}\;  
           \lb 
                \mathbf{1}_{T_k}\lc j\rc \cdot \lb W^{j, k} f\lb X\rb\rb  \,+\, \mathbf{1}_{T_k^c}\lc j\rc \cdot \lb W^{j, k} f\lb X\rb\rb^T
            \rb
         \rb
    \end{align*}
    \begin{align*}
        &
         \underbrace{\;\leq\;}_\textit{Lemma (\ref{lem214})} 
            \underset{j\in T_k \backslash \ls 1\rs}{\prod}\; \lb \,  
                \dim_\textit{row}\lb W_{j, k}\rb \cdot sep-rank\lb W^{j, k} f\lb X\rb\rb
            \,\rb
        \\ &\quad \quad  \quad
            \,\cdot \,
            \underset{j\in T_k^c \backslash \ls 1\rs}{\prod}\; \lb \,  
                \dim_\textit{col}\lb X\rb \cdot sep-rank\lb \lb W^{j, k} f\lb X\rb\rb^T \rb
            \,\rb
        \\ & \quad\quad\quad
            \,\cdot\, 
            sep-rank\lb  \mathbf{1}_{T_k}\lc 1\rc \cdot \lb W^{1, k} f\lb X\rb\rb  \,+\, \mathbf{1}_{T_k^c}\lc 1\rc \cdot \lb W^{1, k} f\lb X\rb\rb^T\rb
    \end{align*}
    \begin{align*}
        & 
        \;=\; 
            \lb \dim_\textit{col}\lb f\lb X\rb\rb\rb^{\abs{T_k^c \backslash \ls 1\rs}}
            \, \cdot \, 
            \lb \,\underset{j\in T_k \backslash \ls 1\rs}{\prod}\; \dim_\textit{row}\lb W_{j, k}\rb \rb 
        \\ & \quad\quad
            \,\cdot\, 
            \lb \underset{j\in T_k \backslash \ls 1\rs}{\prod}\;sep-rank\lb W^{j, k} f\lb X\rb\rb \rb 
            \,\cdot \,
             \lb \,\underset{j\in T_k^c \backslash \ls 1\rs}{\prod}\;  sep-rank\lb \lb W^{j, k} f\lb X\rb\rb^T \rb\,\rb
        \end{align*}
        \begin{align*}
        & \quad\quad
            \,\cdot\, 
            \lb 
                \mathbf{1}_{T_k}\lc 1\rc \cdot sep-rank\lb \lb W^{1, k} f\lb X\rb\rb\rb 
                \,+\, 
                \mathbf{1}_{T_k^c}\lc 1\rc \cdot sep-rank\lb \lb W^{1, k} f\lb X\rb\rb^T\rb
            \rb 
        \end{align*}
        \begin{align*}
        & 
            \underbrace{=}_{Lemma (\ref{lem225})} 
            \lb \dim_\textit{col}\lb f\lb X\rb\rb\rb^{\abs{T_k^c \backslash \ls 1\rs}}
        \\ & \quad\quad\quad\;\;
            \, \cdot \, 
            \lb \,\underset{j\in T_k \backslash \ls 1\rs}{\prod}\; \dim_\textit{row}\lb W_{j, k}\rb \rb 
        \\ & \quad\quad\quad\;\;
            \,\cdot\, 
            \lb \underset{j\in T_k \backslash \ls 1\rs}{\prod}\;sep-rank\lb W^{j, k} X\rb \rb 
        \\ & \quad\quad\quad\;\;
            \,\cdot \,
             \lb \,\underset{j\in T_k^c \backslash \ls 1\rs}{\prod}\;  sep-rank\lb W^{j, k} f\lb X\rb \rb\,\rb
        \\ & \quad\quad\quad\;\;
            \,\cdot\, 
            \lb 
                \mathbf{1}_{T_k}\lc 1\rc \cdot sep-rank\lb W^{1, k} f\lb X\rb\rb 
                \,+\, 
                \mathbf{1}_{T_k^c}\lc 1\rc \cdot sep-rank\lb W^{1, k} f\lb X\rb\rb
            \rb 
    \end{align*}
    \begin{align*}
        & =\;\;\;\;\,
            \lb \dim_\textit{col}\lb X\rb\rb^{\abs{T_k^c \backslash \ls 1\rs}}
            \, \cdot \, 
            \lb \,\underset{j\in T_k \backslash \ls 1\rs}{\prod}\; \dim_\textit{row}\lb W_{j, k}\rb \rb 
        \\ & \quad\quad
            \,\cdot \,
            \lb \,\overset{d}{\underset{j=2}{\prod}}\;  sep-rank\lb W^{j, k} f\lb X\rb \rb\,\rb
        \\ & \quad\quad
            \,\cdot\,
            sep-rank\lb W^{1, k} f\lb X\rb\rb 
        \end{align*}
        \begin{align*}
        & =\;\;\, 
            \lb \dim_\textit{col}\lb X\rb\rb^{\abs{T_k^c \backslash \ls 1\rs}}
            \, \cdot \, 
            \lb \,\underset{j\in T_k \backslash \ls 1\rs}{\prod}\; 
            \dim_\textit{row}\lb W_{j, k}\rb \rb 
            \,\cdot \,
            \lb \,\overset{d}{\underset{j=1}{\prod}}\;  sep-rank\lb W^{j, k} f\lb X\rb \rb\,\rb
        \\ & \quad\quad
        \underbrace{\leq\;\;\;}_{Lemma (\ref{lem21})} 
        \lb \dim_\textit{col}\lb f\lb X\rb\rb\rb^{\abs{T_k^c \backslash \ls 1\rs}}
        \, \cdot \, 
        \lb \,\underset{j\in T_k \backslash \ls 1\rs}{\prod}\; \dim_\textit{row}\lb W_{j, k}\rb \rb 
        \\ &  \quad\quad\quad\quad\quad\quad\quad\quad\quad
              \quad\quad\quad\quad\quad\quad\quad\quad
        \,\cdot \,
        \lb \,\overset{d}{\underset{j=1}{\prod}}\; \dim_\textit{col}\lb W^{j, k}\rb \cdot sep-rank\lb f\lb X\rb \rb\,\rb
        \end{align*}
        \begin{align*}
         & 
        \;=\;\; 
        \lb \,\underset{j\in T_k \backslash \ls 1\rs}{\prod}\; \dim_\textit{row}\lb W_{j, k}\rb \rb 
        \,\cdot \,
        \lb \,\overset{d}{\underset{j=1}{\prod}}\; \dim_\textit{col}\lb W^{j, k}\rb \,\rb  
        \\ & \quad\quad\quad\quad\;\;
        \cdot
        \lb \dim_\textit{col}\lb f\lb X\rb\rb\rb^{\abs{T_k^c \backslash \ls 1\rs}}
        \, \cdot \, 
        \lb sep-rank\lb f\lb X\rb \rb\,\rb^d
    \end{align*}
    Writing again for clarity we have the following two inequalities 
    \equ{\label{670}
        sep-rank\lb L_{H}^{R, d}\circ f\lb X\rb\rb 
        \;\leq\;
        \dim_\textit{col}\lb W_O\rb \cdot
        \overset{H}{\underset{k=1}{\Sigma}}\;\,
        \Delta_k
        \;+\; sep-rank\lb f\lb X\rb\rb
    }
    And
    \begin{equation*}\label{eq680}
        \begin{split}
            & 
            \Delta_k 
            \;\leq\;
            \\ & \quad\quad
            \lb \,\underset{j\in T_k \backslash \ls 1\rs}{\prod}\; \dim_\textit{row}\lb W_{j, k}\rb \rb 
            \,\cdot \,
            \lb \,\overset{d}{\underset{j=1}{\prod}}\; \dim_\textit{col}\lb W^{j, k}\rb \,\rb  
            \\ & \quad\quad
            \cdot
            \lb \dim_\textit{col}\lb f\lb X\rb\rb\rb^{\abs{T_k^c \backslash \ls 1\rs}}
            \, \cdot \, 
            \lb sep-rank\lb f\lb X\rb \rb\,\rb^d            
        \end{split}
    \end{equation*}
    Which is just the first promise given in equations (\ref{eq63}) and (\ref{eq640}) of the lemma, now suppose that the assumption of the same dimensions given in equation 
    (\ref{660}) holds then by the notations given in the lemma body we have 
    \equ{\label{eq690}
        \forall i, k \quad \dim_\textit{col}\lb W^{j, k}\rb = n
        \quad\quad\bigwedge\quad\quad
        \dim_\textit{col}\lb f\lb X\rb\rb = m 
    }
    Combining equations (\ref{eq680}) and (\ref{eq690}) together we get 
    \begin{align*}
        & \Delta_k 
        \;\leq\;\quad\quad
        \\ & \quad\quad\quad
        \lb \,\underset{j\in T_k \backslash \ls 1\rs}{\prod}\; \dim_\textit{row}\lb W_{j, k}\rb \rb 
        \,\cdot \,
        \lb \,\overset{d}{\underset{j=1}{\prod}}\; \dim_\textit{col}\lb W^{j, k}\rb \,\rb  
        \\ & \quad\quad\quad
        \cdot
        \lb \dim_\textit{col}\lb f\lb X\rb\rb\rb^{\abs{T_k^c \backslash \ls 1\rs}}
        \, \cdot \, 
        \lb sep-rank\lb f\lb X\rb \rb\,\rb^d
        \\&\quad
            \;=\; 
            \lb \,\underset{j\in T_k \backslash \ls 1\rs}{\prod}\; m\rb 
            \,\cdot \,
            \lb \,\overset{d}{\underset{j=1}{\prod}}\; n \,\rb  \cdot
            m^{\abs{T_k^c \backslash \ls 1\rs}}
            \, \cdot \, 
            \lb sep-rank\lb f\lb X\rb \rb\,\rb^d
        \\&\quad 
            \;=\;
            m^{\abs{T_k \backslash \ls 1\rs}} 
            \,\cdot \, n^d \, \cdot
            m^{\abs{T_k^c \backslash \ls 1\rs}}
            \, \cdot \, 
            \lb sep-rank\lb f\lb X\rb \rb\,\rb^d
        \\&\quad 
            \;=\; 
            m^{\abs{T_k \backslash \ls 1\rs}\,+\,\abs{T_k^c \backslash \ls 1\rs}} 
            \,\cdot \, n^d \, \cdot \, 
            \lb sep-rank\lb f\lb X\rb \rb\,\rb^d
        \\ & \quad
            \;=\; 
                m^{d-1} \,\cdot \, n^d \, \cdot \, \lb sep-rank\lb f\lb X\rb \rb\,\rb^d
    \end{align*}
    Writing again for clarity we end with 
    \equ{\label{700}
        \Delta_k \;\leq\; m^{d-1} \,\cdot \, n^d \, \cdot \, \lb sep-rank\lb f\lb X\rb \rb\,\rb^d
    }
    Substituting the last (\ref{700}) equation back into equation (\ref{670}) we get 
    \begin{align*}\label{710}
        & sep-rank\lb L_{H}^{R, d}\circ f\lb X\rb\rb 
        \;\leq\;
        \dim_\textit{col}\lb W_O\rb \cdot
        \overset{H}{\underset{k=1}{\Sigma}}\;\,
        \Delta_k
        \;+\; sep-rank\lc f\lb X\rb\rc
    \end{align*}
    \begin{align*}
        &\underbrace{\leq}_\textit{Equation (\ref{700})} 
        \dim_\textit{col}\lb W_O\rb \cdot
        \overset{H}{\underset{k=1}{\Sigma}}\;\,
         m^{d-1} \,\cdot \, n^d \, \cdot \, \lb sep-rank\lc f\lb X\rb \rc\,\rb^d
        \;+\; sep-rank\lc f\lb X\rb\rc
    \end{align*}
    \begin{align*}
        &\;=\; 
        \dim_\textit{col}\lb W_O\rb \cdot
        H \cdot m^{d-1} \,\cdot \, n^d \, \cdot \, \lb sep-rank\lc f\lb X\rb \rc\,\rb^d
        \;+\; sep-rank\lc f\lb X\rb\rc
    \end{align*}
    \begin{align*}
        & \;\leq\; 
        \max\lb n,m\rb \cdot
        H \cdot m^{d-1} \,\cdot \, n^d \, \cdot \, \lb sep-rank\lc f\lb X\rb \rc\,\rb^d
        \;+\; sep-rank\lc f\lb X\rb\rc
        \\& 
        \;\leq\;
        \lb \max\lb n,m\rb \cdot
        H \cdot m^{d-1} \,\cdot \, n^d \, + 1\rb \cdot \, \lb sep-rank\lc f\lb X\rb \rc\,\rb^d
        \\ &
        \underbrace{\leq\;\;\;\;}_{\min\lb m, n\rb \geq 2} 
        \lb \max\lb n,m\rb\cdot \min\lb m, n\rb \cdot
        H \cdot m^{d-1} \,\cdot \, n^d \rb \cdot \, \lb sep-rank\lc f\lb X\rb \rc\,\rb^d
        \\&
        =\;
        \lb m \cdot n \cdot
        H \cdot m^{d-1} \,\cdot \, n^d\rb \cdot \, \lb sep-rank\lc f\lb X\rb \rc\,\rb^d
        \\&
        =\;
        H \cdot m^{d} \,\cdot \, n^{d+1} \cdot \, \lb sep-rank\lc f\lb X\rb \rc\,\rb^d
    \end{align*}
    Altogether we have 
    \equ{
        sep-rank\lb L_{H}^{R, d}\circ f\lb X\rb\rb 
        \leq 
        H \cdot m^{d} \,\cdot \, n^{d+1} \cdot \, \lb sep-rank\lc f\lb X\rb \rc\,\rb^d
    }
    Which gives us the second promise of the lemma, as given in equation (\ref{660}) $\quad\quad\quad\quad\blacksquare$    
\end{proof}
