# Supplementary material for: Transformer Vs. MLP-Mixer: Exponential Expressive Gap For NLP Problems
Source: arXiv:2208.08191 source file (2022-11-17)
Supplement: Supplementary file 6 [file appendix_E.tex]

\section{Transformer lower bound}
\subsection{Theorem 5.5}
\begin{theorem}\label{thm_66_2}
    For $p < \log_3 m$, there is weights assignment, such that, our upper bound 
    \equ{\label{eq860}
        \log_3\; sep-rank\lb y_{p, H}^{R}\rb
        \;\leq\;
        3^p \cdot \lc \log_3 \lb 2 H\rb  + 2\log_3 m \,+ \, 2 \log_3 n \rc
    }
    Is asymptotically tight, in the sense 
   \begin{equation*}
        \begin{split}\label{eq870}
            & \underbrace{3^{p-2}\lb \log_3 \lb m-H\rb + a\rb}_\textit{Lower Bound For Some Weights Assignment}
            \;\leq\;
             \log_3 sep-rank\lb y_{p, H}^{R, 3}\rb
             \quad\quad\quad\quad\quad\quad\quad\quad\quad\quad\quad\quad
            \\ & \quad\quad\quad\quad\quad\quad\quad\quad
                 \quad\quad\quad\quad\quad\quad\quad\quad
            \;\leq\;
            \underbrace{3^p \cdot \lc \log_3 \lb 2 H\rb  + 2\log_3 m \,+ \, 2 \log_3 n \rc}_\textit{Our Upper Bound}   
        \end{split}
    \end{equation*}
\end{theorem}

\begin{proof}
    See theorem (7.1), from the book (\cite{levine2022tensors}).
    $\quad\quad\blacksquare$
\end{proof}
