# Supplementary material for: Transformer Vs. MLP-Mixer: Exponential Expressive Gap For NLP Problems
Source: arXiv:2208.08191 source file (2022-11-17)
Supplement: Supplementary file 7 [file appendix_F.tex]

\section{Main theorem}
\subsection{Theorem 3.3 \& conclusion 5.6}
\begin{theorem}
    Let $\mathcal{F}_{B, p}^{T}$ be the class of all the transformers architectures. With up to
    $B$ parameters, and depth $p$. 
    And let $\mathcal{F}_{B, p}^{MM}$ be the class of all the mlp-architectures. 
    Possibly with permutations of the input before each mlp-layer. And with up to $B$ parameters, 
    and depth $p$.
    Then we have the following asymptotic relation 
    $\frac{\log\lb\; inf-sep\lb \mathcal{F}_{B}^{T}\rb\;\rb\;\;}{ 
     \log\lb\; sup-sep\lb \mathcal{F}_{B}^{MM}\rb\rb}
     = \Omega\lb \lb \frac{3}{2}\rb^{p}\rb$.
     And more formally we have $\mathcal{F}_{B, p}^{MM} \prec_{\lb \frac{3}{2}\rb^p} \mathcal{F}_{B, p}^{T}$.
\end{theorem}

\begin{conclusion}\label{c1_2}
    We got, that for $\mathcal{F}_{B}^{T},\, \mathcal{F}_{B}^{mlp}$ 
    the classes of, transformer and mlp-based architectures,  
    with up to $B$ parameters 
    respectively.
    It holds that,   
    $\frac{\log_3 \sup-sep\lb \mathcal{F}_{B}^{T}\rb}
    {\log_3 \inf-sep\lb \mathcal{F}_{B}^{mlp}\rb} \,=\,
    \Omega\lb\, \lb \frac{3}{2}\rb^p \,\rb$. 
    Or more formally, there is dominance relation of the form
    $\mathcal{F}_{B}^{mlp} \prec_{\lb \frac{3}{2}\rb^p} \mathcal{F}_{B}^{T}$ .
\end{conclusion}

\begin{proof}
    Using the class of functions dominance definition, 
    we want to show that for $p\,=\,f\lb B\rb$ 
    for some monotonic increasing function 
    $f:\mathbb{N} \to \mathbb{N}$ 
    with 
    $\underset{n \to \infty}{\lim} \, f\lb n\rb = \infty$
    it holds that, 
    $\frac{\log_3 \inf-sep\lb \mathcal{F}_{B}^{T}\rb}
    {\log_3 \sup-sep\lb \mathcal{F}_{B}^{mlp}\rb} \,=\,
    \Omega\lb\, \lb \frac{3}{2}\rb^p \,\rb$, 
    hence, in order to stay in the depth efficiency regime 
    of both architectures, we will limit the depth growth to satisfy
    $p < \log_3 m$.  
    and will use the following reasonable assumptions, 
    about the dimensions of the architecture
    $n < m^4$ and $H < \frac{m}{2}$ when taking $p\to \infty$. 
    \paragraph{}
    Using lemma (\ref{ub_lemma}) we have 
    \begin{equation}\label{eq_ub_2_5}
        \log_3 \; 
        \sup-sep\lb y_{p, H}^{R, MM}\rb
        \;\leq\;
        11 \,\cdot\, 2^{p} \log_3 m         
    \end{equation}
    While from lemma (\ref{lb_lemma}) we have 
    \begin{equation}\label{eq_up_2_5}
        \log_3 \; \inf-sep\lb y_{p, H}^{R, T}\rb
        \;\geq\;
         3^{p-3}\log_3 m                            
    \end{equation}
    Finally combining equations (\ref{eq_up_2_4}) and (\ref{eq_ub_2_4}) we have 
    \begin{align*}
        \frac{\log_3 sep-rank\lb y_{p, H}^{R, T}\rb}{ 
              \log_3 sep-rank\lb y_{p, H}^{R, MM}\rb}
        \;\geq\; 
        \frac{3^{p-3}\,\log_3 m}{11 \cdot 2^p \log_3 m}
        \;=\; \Omega\lb \lb \frac{3}{2}\rb^p\rb     
    \end{align*}
    Which gives exponential gap, between the transformer, to the mlp-based architectures.
    Finally combining equations
    (\ref{eq_up_2_5}) and (\ref{eq_ub_2_5}) 
    we have 
    \begin{align*}
        \frac{
        \log_3\, \inf-sep-rank\lb y_{p, H}^{R, T}\rb}{
        \log_3\, \sup-sep-rank\lb y_{p, H}^{R, MM}\rb}
        \;\geq\; 
        \frac{3^{p-3}\,\log_3 m}{11 \cdot 2^p \log_3 m}
        \;=\; \Omega\lb \lb \frac{3}{2}\rb^p\rb     
    \end{align*}
    which gives exponential gap between the transformer to the mlp-based 
    architectures. $\quad\blacksquare$
\end{proof}
