# Supplementary material for: Transformer Vs. MLP-Mixer: Exponential Expressive Gap For NLP Problems
Source: arXiv:2208.08191 source file (2022-11-17)
Supplement: Supplementary file 8 [file appendix_G.tex]

\section{Depth efficiency regime result}
\subsection{Conclusion 5.7}
\begin{conclusion}\label{c2_2}
    If $p < \log_3 m$, and assuming 
    $p >> \log_3\log_3 m\;$ $n < m^2$,
    $H < \frac{m}{2}$ and $p \geq 13$. 
    Then, every mlp-based architecture, have strictly smaller expressive power in modeling 
    multi-variable dependencies, then any attention based architecture, 
    when fixing the depth and parameters budget.
    Also, for $\log_3 m < p < \log_2 m$,
    then still, transformers enjoy strictly higher expressive power. Then mlp-based architectures, for large enough $p$.
    And when moving, into the depth efficiency regime,
    $p < \log_3 m$.
    The gap becomes asymptotically exponential in $p$.    
\end{conclusion}
\subsection{Proof}
\begin{proof}
        We will do cases analysis: \\
    \textbf{Case-1:} $\quad p < \log_3 m\quad$ we will also assume $H < \frac{m}{2}$ and $n < m^2$ and $9 < m$ since those are reasonable assumption about the number of heads
    \paragraph{}
    Using equation (\ref{eq730}) from theorem (\ref{229}) we have  
    \begin{align*}
        sep-rank\lb y_{p, H}^{R, MM}\rb
        \;\leq\;
        \lb 2 H \cdot m^2 \,\cdot \, n^2\rb^{2^p}        
    \end{align*}
    taking $\log_3$ we end with
    \equ{\label{eq930}
        \log_3 sep-rank\lb y_{p, H}^{R, MM}\rb
        \;\leq\;
        2^p \lc \log_3 \lb 2 H\rb \,+\, 2\log_3 m \,+ \, 2 \log_3 n \rc
    }
    while from equation (\ref{eq870}) we have
    \equ{\label{eq940}
        \underbrace{3^{p-2}\lb \log_3 \lb m-H\rb + a\rb}_\textit{Lower Bound For Some Weights Assignment}
        \;\leq\;
         \log_3 sep-rank\lb y_{p, H}^{R, T}\rb
    }
    Combining equations (\ref{eq940}) and (\ref{eq930}) together it is enough to show 
    \equ{\label{eq950}
         2^p \lc \log_3 \lb 2 H\rb \,+\, 2\log_3 m \,+ \, 2 \log_3 n \rc
         \;\leq\; 
         3^{p-2}\lb \log_3 \lb m-H\rb + a\rb
    }
    in order to show 
    \begin{align*}
        \log_3\lb  sep-rank\lb y_{p, H}^{R, MM}\rb\rb  
        \;\leq\;
         \log_3 \lb sep-rank\lb y_{p, H}^{R, Tr}\rb\rb
    \end{align*}
    so lets turn into proving equation (\ref{eq950}) 
    \begin{align*}
         2^p \lc \log_3 \lb 2 H\rb \,+\, 2\log_3 m
                  \,+ \, 2 \log_3 n \rc
         \;\leq\; 
         3^{p-2}\lb \log_3 \lb m-H\rb + a\rb
    \end{align*}
    \begin{align*}
        \Uparrow        
    \end{align*}
    \begin{align*}
        2^p \log_3 \lb 2 H  m^2 n^2\rb 
        \;\leq\; 
        3^{p-2} \log_3 \lb m-H\rb        
    \end{align*}
    \begin{align*}
        \Uparrow        
    \end{align*}
    \begin{align*}
         p \log_3 2 + \log_3\log_3 \lb 2 H  m^2 n^2\rb 
         \;\leq\; 
         p - 2 +  \log_3\log_3 \lb m-H\rb
    \end{align*}
    \begin{align*}
        \Uparrow
    \end{align*}
    \begin{align*}
         2 +  \log_3\frac{\log_3 \lb 2 H  m^2 n^2\rb}{\log_3 \lb m-H\rb} 
         \;\leq\; 
         p \lb \log_3 \,3 - log_3 \,2\rb
    \end{align*}
    \begin{align*}
        \Uparrow
    \end{align*}
    \begin{align*}
         2 +  \log_3\frac{\log_3 \lb 2 H  m^2 n^2\rb}{\log_3 \lb m-H\rb} 
         \;\leq\; 
         p \, \log_3 \,\frac{3}{2}
    \end{align*}
    \begin{align*}
        \Uparrow \quad \textit{since} \; H < \frac{m}{2} < \frac{2 m}{3}
    \end{align*}
    \begin{align*}
        2 +  \log_3\frac{\log_3 \lb m^3 n^2\rb}{\log_3 \lb m\rb - 1}
         \;\leq\; 
         p \, \log_3 \,\frac{3}{2}
    \end{align*}
    \begin{align*}
        \Uparrow \quad \textit{since} \; n < m^2 
    \end{align*}
    \begin{align*}
         2 +  \log_3 \lb 7 
         \frac{\log_3 \lb m\rb}{\log_3 \lb m\rb - 1} \rb 
         \;\leq\; 
         p \, \log_3 \,\frac{3}{2}
    \end{align*}
    \begin{align*}
        \Uparrow \quad \textit{since} \; n < m^2 
    \end{align*}
    \begin{align*}
        \frac{2 +  \log_3 7}{\log_3 \frac{3}{2}} 
        + 
        \frac{1}{\log_3 \frac{3}{2}} \log_3 \lb 1 + \frac{1}{\log_3 \lb m\rb - 1} \rb 
         \;\leq\; 
         p 
    \end{align*}
    \begin{align*}
        \Uparrow \quad \textit{since} \; \log\lb 1 + x\rb \leq x 
    \end{align*}
    \begin{align*}
        \frac{2 +  \log_3 7}{\log_3 \frac{3}{2}} 
        + 
        \frac{1}{\log_3 \frac{3}{2}}  \frac{1}{\log_3 \lb m\rb - 1}  
         \;\leq\; 
         p 
    \end{align*}
    \begin{align*}
        \Uparrow \quad \textit{since} \; m \geq 9 
    \end{align*}
    \begin{align*}
        p \geq  \frac{3 +  \log_3 7}{\log_3 \frac{3}{2}} \approx 12.9
    \end{align*}
    Hence we show that at least for every $p\geq 13$ then degree $3$ transformers have strictly larger expressive power, then squared ones, and although this $p$ may be 
    to large in practice, it still meaningful in the asymptotic sense, and the limit isn't too far in the infinity.\\
    \textbf{Case-2:} $\quad p > \log_3 m \quad$ and like before we also assume $H < \frac{m}{2}$ and $n < m^2$
    \paragraph{}
    In this case \cite{levine2020limits} provides the lower bound
    \begin{align*}
        \log_3 sep-rank\lb y_{p, H}^{R, Tr}\rb
        = \Omega\lb p \lb m-H\rb\rb          
    \end{align*}

    hence
    \begin{align*}
        \log_3\lb  sep-rank\lb y_{p, H}^{R, MM}\rb\rb  
        \;\leq\;
         \log_3 \lb sep-rank\lb y_{p, H}^{R, Tr}\rb\rb
    \end{align*}
    \begin{align*}
        \Uparrow
    \end{align*}
    \begin{align*}
         2^p \lc \log_3 \lb 2 H\rb \,+\, 2\log_3 m \,+ \, 2 \log_3 n \rc
         \;\leq\; 
         C p\lb m-H\rb
    \end{align*}
    \begin{align*}
        \Uparrow \quad \textit{since}\quad H < \frac{m}{2}
    \end{align*}
    \begin{align*}
         2^p \lc \log_3 \lb m\rb \,+\, 2\log_3 m \,+ \, 4 \log_3 m \rc
         \;\leq\; 
         C p\lb \frac{m}{2}\rb
    \end{align*}
    \begin{align*}
        \Uparrow \quad \textit{since}\quad \log_3 m < p
    \end{align*}
    \begin{align*}
        2^p \lc \log_3 \lb m\rb 
                 \,+\, 2\log_3 m 
                 \,+ \, 4 \log_3 m 
            \rc
         \;\leq\; 
         C \log_3 m\lb \frac{m}{2}\rb
    \end{align*}
    \begin{align*}
        \Uparrow
    \end{align*}
    \begin{align*}
         7 \cdot 2^p
         \;\leq\; 
         \frac{C}{2} \cdot m
    \end{align*}
    \begin{align*}
        \Uparrow
    \end{align*}
    \begin{align*}
        p
         \;\leq\; 
         \log_2 \frac{C}{14} + \log_2 m
    \end{align*}
    \begin{align*}
        \Uparrow
    \end{align*}
    \begin{align*}
        p
        \;\leq\; 
        \log_2 m
    \end{align*}
    \\\textbf{Case-3:} 
    $\quad p < \log_3 m\quad$ in addition to  $n < m^2$ and $H < \frac{m}{2}$ when taking $p\to \infty$. \\
    Using lemma (\ref{ub_lemma}) we have 
    \begin{equation}\label{eq_ub_2_4}
        \log_3 \; 
        \sup-sep\lb y_{p, H}^{R, MM}\rb
        \;\leq\;
        11 \,\cdot\, 2^{p} \log_3 m         
    \end{equation}
    While from lemma (\ref{lb_lemma}) we have 
    \begin{equation}\label{eq_up_2_4}
        \log_3 \; \inf-sep\lb y_{p, H}^{R, T}\rb
        \;\geq\;
         3^{p-3}\log_3 m                            
    \end{equation}
    Finally combining equations (\ref{eq_up_2_4}) and (\ref{eq_ub_2_4}) we have 
    \begin{align*}
        \frac{\log_3 sep-rank\lb y_{p, H}^{R, T}\rb}{ 
              \log_3 sep-rank\lb y_{p, H}^{R, MM}\rb}
        \;\geq\; 
        \frac{3^{p-3}\,\log_3 m}{11 \cdot 2^p \log_3 m}
        \;=\; \Omega\lb \lb \frac{3}{2}\rb^p\rb     
    \end{align*}
    Which gives exponential gap, between the transformer, to the mlp-based architectures. $\quad\blacksquare$
\end{proof}
