# Supplementary material for: Transformer Vs. MLP-Mixer: Exponential Expressive Gap For NLP Problems
Source: arXiv:2208.08191 source file (2022-11-17)
Supplement: Supplementary file 9 [file appendix_H.tex]

\section{$2^\alpha$ proposition}
\subsection{Proposition 5.8}
\begin{proposition}\label{p1_2}
    Conclusion (\ref{c1_2}), states dominance relation,
    between transformer and mlp classes, with the same depth. 
    When comparing, classes of different depth
    $\mathcal{F}_{B,\, p_{n, mlp}}^{mlp},
    \;\mathcal{F}_{B,\, p_{n, T}}^{T}$
    Then as long as 
    $\alpha = \underset{n\to \infty}{\limsup}
    \;\frac{p_{n, mlp}}{p_{n, T}} 
    < \log_2 3 \simeq 1.584$. 
    Then, the following, dominance relation, still holds, 
    $\mathcal{F}_{B, p_m}^{mlp} \prec_{\lb \frac{3}{2^\alpha}\rb^p} \mathcal{F}_{B, p_t}^{T}$.    
\end{proposition} 
\subsection{Proof}
\begin{proof}
    Using the class of functions dominance definition. 
    We are interested to show that for $\;p\,=\,f\lb B\rb$,  
    for some monotonic increasing function 
    $f:\mathbb{N} \to \mathbb{N}$ 
    with 
    $\underset{n \to \infty}{\lim} \, f\lb n\rb = \infty$
    it holds that, 
    $\frac{\log_3 \inf-sep\lb \mathcal{F}_{B}^{T}\rb}
    {\log_3 \sup-sep\lb \mathcal{F}_{B}^{mlp}\rb} \,=\,
    \Omega\lb\, \lb \frac{3}{2^\alpha}\rb^p \,\rb$. 
    We will take $p_{n, T}<\log_3 d$ in order to stay, 
    in the depth efficiency regime of both architectures.
    We will also use the following reasonable assumptions, 
    about the dimensions of the architecture
    $n < m^4$ and $H < \frac{m}{2}$
    when taking $p\to \infty$. 
    Using lemma (\ref{ub_lemma}) we have 
    \begin{equation}\label{eq_ub_2_3}
        \log_3 \; 
        \sup-sep\lb y_{p_{n, mlp}, H}^{R, MM}\rb
        \;\leq\;
        11 \,\cdot\, 2^{p_{n, mlp}} \log_3 m         
    \end{equation}
    While from lemma (\ref{lb_lemma}) we have 
    the following lower bound
    \begin{equation}\label{eq_up_2_3}
        \log_3 \; \inf-sep\lb y_{p_{n, T}, H}^{R, T}\rb
        \;\geq\;
         3^{p_{n, T}-3}\log_3 m                            
    \end{equation}
    Finally combining equations (\ref{eq_up_2_3}) and (\ref{eq_ub_2_3}) 
    we have 
    \begin{align*}
    & 
        \frac{
        \log_3\,
        \inf-sep-rank\lb y_{p_{n, T}, H}^{R, T}\rb}{
        \log_3\, 
        \sup-sep-rank\lb y_{p_{n, mlp}, H}^{R, MM}\rb}
        \;\geq\; 
        \frac{3^{p_{n, T}-3}\,\log_3 m}{11 \cdot 2^{p_{n, mlp}} \log_3 m}
        \;=\;
        \Omega\lb 
            \frac{3^{p_{n, T}}}{2^{p_{n, mlp}}}
        \rb
    \\ & 
        \;=\; \Omega\lb 
                \lb 
                \frac{3}{2^{\frac{p_{n, mlp}}{p_{n, T}}}}
                \rb^{p_{n, T}}
        \rb
        \;=\; \Omega\lb 
                \lb 
                \frac{3}{2^{\underset{n\to \infty}{\limsup}\;
                \frac{p_{n, mlp}}{p_{n, T}}}}
                \rb^{p_{n, T}}
        \rb
        \;=\; \Omega\lb 
                \lb 
                \frac{3}{2^\alpha}
                \rb^{p_{n, T}}
        \rb
    \end{align*}
    Which is just the desired exponential gap between the transformer to the mlp-based 
    architectures.$\quad\blacksquare$ 
\end{proof}

\begin{lemma}\label{lb_lemma}
    For $y_{p, H}^{R, T}$ transformer architecture, 
    with residual connection, transposes, and multi-head attentions, without activations and normalization layers. 
    With the following choices $p < \log_3 m$, $n < m^4$ 
    , $H < \frac{m}{2}$
    the following lower bound holds, 
    \begin{equation}\label{eq_ub_4}
        \log_3 \; \inf-sep\lb y_{p, H}^{R, T}\rb
        \;\geq\;
         3^{p-3}\log_3 m            
    \end{equation}
\end{lemma}
\begin{proof}
    Using equation (\ref{eq870}) we have
    \equ{\label{eq940_4}
        3^{p-2}\lb \log_3 \lb m-H\rb + a\rb
        \;\leq\;
         \log_3 sep-rank\lb y_{p, H}^{R, T}\rb
    }
    Hence 
    \begin{align*}
        & 
        \log_3 sep-rank\lb y_{p, H}^{R, T}\rb
        \;\geq\;
        3^{p-2}\lb \log_3 \lb m-H\rb + a\rb
        \;\geq\;
        3^{p-2} \log_3 \lb m-H\rb
        \\ & 
        \underbrace{\;\geq\;}_{H < \frac{m}{2}}
        3^{p-2} \log_3 \lb \frac{m}{2}\rb
        \underbrace{\;\geq\;}_\textit{$\log$-concavity}
        3^{p-2} \frac{\log_3 \lb m\rb}{2}
        \;\geq\;
        3^{p-2} \frac{\log_3 \lb m\rb}{3}
        \;=\; 
        3^{p-3} \log_3 \lb m\rb
    \end{align*}
    So we just ended with the following lower bound 
    \begin{equation}\label{eq_lb_4}
        \log_3 sep-rank\lb y_{p, H}^{R, T}\rb
        \;\geq\;
         3^{p-3}\log_3 m            
    \end{equation}
    As was claimed $\QED$
\end{proof}

    
\begin{lemma}\label{ub_lemma}
    For $y_{p, H}^{R, MM}$ mlp-based architecture, 
    with residual connection, transposes, permutations 
    and $\sigma_2$-activations. 
    Without activations and normalization layers. 
    With the following choices $p < \log_3 m$, $n < m^4$.
    The following upper-bound holds
    \begin{equation}\label{eq_ub_4}
        \log_3 \; 
        \sup-sep\lb y_{p, H}^{R, MM}\rb
        \;\leq\;
        11 \,\cdot\, 2^{p} \log_3 m         
    \end{equation}
\end{lemma}
\begin{proof}
    Using equation (\ref{eq930}), we have 
    \begin{align*}
        \log_3 sep-rank\lb y_{p, H}^{R, MM}\rb
        \;\leq\;
        2^{p} \lc 
        \log_3 \lb 2 H\rb \,+\, 2\log_3 m \,+ \, 2 \log_3 n \rc
    \end{align*}
    Hence 
    \begin{align*}
        & 
        \log_3 
        sep-rank\lb y_{p, H}^{R, MM}\rb
        \;\leq\;
        2^{p} 
        \lc \log_3 \lb 2 H\rb \,+\, 2\log_3 m \,+ \, 2 \log_3 n \rc
        \\ & \quad\quad\quad\quad\quad
        \underbrace{\;\leq\;}_{n < m^4,\; H < \frac{m}{2}}
        2^{p}   \lc \log_3 \lb 2 \cdot \frac{m}{2}\rb 
                \,+\, 2\log_3 m \,+ \, 2 \log_3 m^4
            \rc
        \\ & \quad\quad\quad\quad
        \;=\;
        2^{p} \lc \log_3 \lb m\rb 
                 \,+\, 2\log_3 m 
                 \,+ \, 8 \log_3 m
            \rc
        \;=\;
        11 \cdot 2^{p} \log_3 m
    \end{align*}
    And overall we ended with the following upper-bound
    \begin{equation}\label{eq_up_2}
        \log_3 \sup-sep\lb y_{p, H}^{R, MM}\rb
        \;\leq\; 
        11 \,\cdot\, 2^{p} \log_3 m 
    \end{equation}
    As was claimed $\QED$ 
\end{proof}
    
