# Supplementary material for: Transformer Vs. MLP-Mixer: Exponential Expressive Gap For NLP Problems
Source: arXiv:2208.08191 source file (2022-11-17)
Supplement: Supplementary file 10 [file appendix_I.tex]

\section{Experiment 6.2 - Depth to width ratio}
\subsection{Experiment theory}
\subsubsection{Transformer optimal depth to width ratio}
\begin{theorem}\label{thm_986}
    The optimal depth to width ratio for transformers 
    architectures is $p\approx\log_3 d$ 
    where $p$ and $d$ denotes the transformer depth and width respectively.
\end{theorem}

\begin{proof}
    Let $\,f\lb p, d\rb\,$ denote the separation-rank\\
    \textbf{Case-1:}
    Then first for the regime 
    $\,p \,<\, \log d\,$,  we have 
    \begin{equation}
        f\lb p, d\rb = 3^p \log d  
    \end{equation}
    fixing the budget we have $C\, p\, d^2 = B$ and hence 
    $p\, d^2 = \frac{B}{C}$ now let $D = \frac{B}{C}$ then we have 
    $d = \sqrt{\frac{D}{p}}$ and hence $f$ can be written as 
    \begin{equation}
        f\lb p\rb
        = 3^p\, \log\, \sqrt{\frac{D}{p}}
        = \frac{3^p}{2}\, \log\, \frac{D}{p}
        = \frac{3^p}{2}\,\lb\, \log D \,-\, \log p\,\rb 
    \end{equation}
    taking the derivative w.r.t $p$ we get 
    \begin{equation}
        \frac{\partial}{\partial p}\; f\lb p\rb
        = 
        \ln 3 \, \frac{3^p}{2}\,\lb\, \log D \,-\, \log p\,\rb
        \,-\,
        \frac{3^p}{2\, p}
        =
        \frac{3^p}{2}\lc 
            \ln 3 \, \log \frac{D}{p} - \frac{1}{p}
        \rc
    \end{equation}
And let us analyze the sign of the derivative then indeed, we have 
\begin{equation}
    \ln 3 \, \log \frac{D}{p} - \frac{1}{p} < 0
    \quad\iff\quad
    \ln 3 \, \log \frac{D}{p} < \frac{1}{p}
    \quad\iff\quad
    \ln 3 \,\log D - \ln 3 \log p < \frac{1}{p}
\end{equation}

\begin{equation}
    \quad\iff\quad
    \ln 3 \,\log D < \frac{1}{p} + \ln 3\, \log p 
    \quad\iff\quad
    \log D < \frac{1}{p\,\ln 3} + \log p 
\end{equation}

\begin{equation}
    \quad\implies\quad
    \log D < 1 + \log p  
    \quad\implies\quad
     D < 2\cdot p
    \quad\underbrace{\;\;\implies\;\;}_{D = p\cdot d^2}\quad
    d^2 < 2
\end{equation}
But $d > 1$ and hence we always have 
\begin{equation}
    \frac{\partial}{\partial p}\, f\lb p\rb > 0
\end{equation}
hence in the region $p<\log d$ then increasing $p$ only increases the expressivity, and hence, 
$p=\log d$ is the best in this region.\\
\textbf{Case-2:} 
The second regime is when $p > \log d$ and for this case we have 
\begin{equation}
    f\lb p, d\rb = d\log d   
\end{equation}
And since $d\log d$ is monotonic increasing function we get, that taking $d$ as large as possible would increase our expressive power, and hence in this regime also we have that $p=\log d$ is the best choice, and overall we have  $p=\log d$ as we claimed. \QED
\end{proof}

\begin{remark}
    The last theorem is based on \cite{levine2020limits}, where they 
    show empirically, that indeed $p=\log_3 d$ is the optimal depth to 
    width ratio, for the transformer architecture.     
\end{remark}

\subsubsection{General architectures - depth to width ratio}
\begin{theorem}
    For every architecture 
    $y_{p, d}$ with 
    %\todo{prove it}
    \equ{
        \log_\alpha\lc\, sep-rank\lb y_{p, d}\rb\,\rc 
        = \Theta\lb \, Q_1\lb p, d\rb \cdot \alpha^{p}\,\rb
    }
    for $p < \log_\alpha d$ and 
    \equ{
        \log_\alpha\lc\, sep-rank\lb y_{p, d}\rb\,\rc 
        = \Theta\lb \, Q_2\lb p, d\rb \,\rb
    }
    for $p> \log_\alpha d$  
    where $Q_1, \, Q_2:\mathbb{N}^2 \to \mathbb{N}$ is some multinomial with finite degree, 
    and $1 < \alpha \in \mathbb{R}$ is the exponent basis then fixing a budget $B$ 
    the optimal depth to width ratio satisfies
    $\frac{p}{\log_\alpha d}>1$.
\end{theorem}
\begin{proof}
    We will show it for each regime separately. \\
    \textbf{Case-1:} $p < \log_\alpha d$, in this case we have, 
    \begin{equation}
        f\lb p, d\rb = Q_1\lb p, d\rb \alpha^p
    \end{equation}
    fixing the budget we have $C p d^2 = B$ and hence 
    $p d^2 = \frac{B}{C}$ now let $D=\frac{B}{C}$ 
    we have 
    \begin{equation}
        d = \sqrt{\frac{D}{p}}
    \end{equation}
    and hence when fixing $B$ we have 
    \begin{equation}
        f\lb p\rb = Q_1\lb\, p,\; \sqrt{\frac{D}{p}}\,\rb\, \alpha^p
    \end{equation}
    Then we have 
    \begin{equation}
        f\lb p\rb \,\approx\, C\, p^{\beta}\, \alpha^p
    \end{equation}
    Where $\beta$ is some constant which may be positive or maybe negative, however it clear, 
    that asymptotically, when the budget is large enough, then taking the maximal $p$ in the regime, 
    which is just $p = \log_\alpha d$ is the best option.\\ 
    \textbf{Case-1:} $p > \log_\alpha d$, in this case we have $f\lb p,\, d\rb = Q_2\lb p,\, d\rb$ 
    however no matter what the best choice are, since its in the regime, for sure we are 
    $p>\log_\alpha d$. \\
    \textbf{Summarizing:} Overall we got that $p>\log_\alpha d$ as we claimed. \QED
\end{proof}
 
\subsubsection{Mixer regime-dependent upper-bounds}
\begin{theorem}
    For mixer architectures, the following bounds hold 
    \equ{
    \log_2\lc\, sep-rank\lb y_{p, d}\rb\,\rc 
    = O\lb \, Q_1\lb p, d\rb \cdot 2^{p}\,\rb
    }
    for $p < \log_\alpha d$ and 
    \equ{
        \log_2 \lc\, sep-rank\lb y_{p, d}\rb\,\rc 
        = O\lb \, Q_2\lb p, d\rb \,\rb
    }   
    for $p > \log_\alpha d$
\end{theorem}

\begin{proof}
    We will divide the proof into proving the $p<\log_\alpha d$
    bound first, and 
    then will turn into proving the bound for the 
    second regime $p>\log_\alpha d$  
    \paragraph{}
    \textbf{Case-1:} $p<\log_\alpha d\;\;$
    As for the upper bound for this case. 
    Then it was already proven, in 
    theorem (\ref{thm57}). And actually, 
    as shown by lemma (\ref{ub_lemma}). It is enough for us,
    in order to get derivation of the desired 
    $O\lb Q_1\lb p, d\rb \cdot 2^p\rb$ form.
    \paragraph{}
    \textbf{Case-2:} $p>\log_\alpha d\;\;$ 
    As for the upper bound for this case. 
    Then starting from first definitions, we have 
    \begin{equation}
        T \,=\, L_p \circ ... \circ L_1\lb X\rb 
    \end{equation}
    Where 
    \equ{
        L_{i}\lb X\rb = 
        \sigma_2\lb \mathbf{1}_O\lc i\rc \cdot W_i^o \pi_e \lb X\rb  
        + \mathbf{1}_E\lc i\rc \cdot \lc W_i^e \pi_o \lb X^T\rb \rc^T \rb
        + \mathbf{1}_R\lc i\rc \pi_r\lb X\rb 
    } 
    Writing differently we have  
    \begin{equation}
        L_{i}\lb X\rb = 
        \lb 
            \mathbf{1}_O\lc i\rc \cdot W_i^o \pi_e \lb X\rb  
            + 
            \mathbf{1}_E\lc i\rc \cdot \lc W_i^e \pi_o \lb X^T\rb
        \rc^T \rb^{\odot 2}
        + \mathbf{1}_R\lc i\rc \pi_r\lb X\rb
    \end{equation}
    When we can think on $\lb L_{i}\rb_{k l}$ as 
    degree 2 multinomial, in $X$ elements. 
    And hence if $f\lb X\rb$ is matrix function s.t 
    $f\lb X\rb_{k l}$ is multinomial, 
    with up to degree $2^{i-1}$ elements, and each element, is combined from one of, the $n \cdot m$ different variables. 
    Then, clearly $L_i\lb f\lb X\rb\rb_{k l}$ is multinom, 
    in $X$ variables, 
    with multinomial degree at most $2^{i}$.
    of the form 
    \begin{align*}
        L_i\lb f\lb X\rb\rb_{k l}
         = 
        \overset{\eta_{p, m, n}}{\underset{i=1}{\Sigma}}  
        \, a_i \, 
        \underset{k,\, l}{\prod}\; x_{k l}^{\alpha_{k l}^i}
    \end{align*}
    Using the separation-rank sub-additive nature we can get 
    \begin{align*}
        &
        \sup-sep \lb L_i\lb f\lb X\rb\rb_{k l}\rb 
         \leq 
        \overset{\eta_{p, m, n}}{\underset{i=1}{\Sigma}}  
        \sup-sep\lb \, a_i \, 
        \underset{k,\, l}{\prod}\; x_{k l}^{\alpha_{k l}^i}
        \rb 
        \\ & 
        = 
        \overset{\eta_{p, m, n}}{\underset{i=1}{\Sigma}}  
        \sup-sep\lb \, a_i \, 
        \lb \underset{k,\, l \in A}{\prod}\; x_{k l}^{\alpha_{k l}^i}\rb 
        \cdot 
        \lb \underset{k,\, l \in B}{\prod}\; x_{k l}^{\alpha_{k l}^i}\rb
        \rb 
        = \eta_{p, m, n}
    \end{align*}
    And since 
    \begin{align*}
        \forall k, l \quad\quad
        \underset{k,\, l}{\Sigma}\; \alpha_{k l}^i 
        \leq degree\lb L_i\lb f\lb X\rb\rb_{k l}\rb \leq 2^i
    \end{align*}
    Then clearly we have 
    \begin{equation}
        \eta_{p, m, n} \leq 
        \gamma_{p, m, n} \defeq \abs{\ls
            \lb a_1, ..., a_{m n}\rb \;|\; 
            \overset{m\cdot n}{\underset{i=1}{\Sigma}}\; a_{i} \leq 2^p
        \rs}
    \end{equation}
    And we are interested with bounding $\gamma_{p, m, n}$, which is just the multi-set 
    coefficient $\binom{n+k-1}{k}$, and in our case
    \begin{equation}
        \gamma_{p, m, n}
         \,=\, \overset{2^p}{\underset{l=1}{\Sigma}}\;
         \binom{l + m \cdot n - 1}{m \cdot n}
         \,\leq\, 2^p \cdot \binom{2^p + m\cdot n}{m \cdot n}
         \,=\, 2^p\frac{\lb 2^p + m\cdot n\rb!}{\lb 2^p\rb! \lb m\cdot n\rb!} 
    \end{equation}
    Using the Sterling approximation we have  
    \begin{align*}
        &
        \gamma_{p, m, n}
        \,\leq\, 
        2^p \frac{
            \sqrt{4\pi \lb 2^p + m\cdot n\rb}\lb \frac{2^p + m\cdot n}{e}\rb^{2^p + m\cdot n}
        }{
            \sqrt{2\pi \lb m\cdot n\rb}\lb \frac{m\cdot n}{e}\rb^{m\cdot n}
            \,\cdot\,  
            \sqrt{2\pi \lb 2^p\rb}\lb \frac{2^p}{e}\rb^{2^p}
        }
        \quad\quad\quad\quad\quad\quad\quad\quad
        \quad\quad\quad\quad\quad\quad
        \quad\quad\quad\quad\quad\quad
        \\ & 
        \quad\quad\;\;\;
        \,=\, 
        2^p \sqrt{\frac{\lb 2^p + m\cdot n\rb}{\pi \lb m\cdot n\rb \cdot 2^p}}
        \frac{\lb \frac{2^p + m\cdot n}{e}\rb^{2^p}}{\lb \frac{2^p}{e}\rb^{2^p}}
        \frac{\lb \frac{2^p + m\cdot n}{e}\rb^{m\cdot n}}{\lb \frac{m\cdot n}{e}\rb^{m\cdot n}}        
        \\&\quad\quad\;\;\;
            \,=\, 
            2^p
            \sqrt{\frac{ 2^p + m\cdot n}{\pi \lb m\cdot n\rb \cdot 2^p}} \, \cdot\,
            \lb \frac{2^p + m\cdot n}{2^p}\rb^{2^p}\, \cdot\,
            \lb \frac{2^p + m\cdot n}{m\cdot n}\rb^{m\cdot n}        
        \\ & \quad\quad\;\;\;
            \,=\,
            \frac{2^p}{\sqrt{\pi}}                    \,\cdot\,
            \sqrt{\frac{1}{2^p}+\frac{1}{m\cdot n}}  \,\cdot\,
            \lb 1+\frac{m\cdot n}{2^p}\rb^{2^p}       \,\cdot\,
            \lb 1+\frac{2^p}{m\cdot n}\rb^{m\cdot n}
        \\ & \quad\quad\;\;\;
            \,\leq\, 
            2^p                                     \,\cdot\,
            1                                        \,\cdot\,
            \lb 1+\frac{m\cdot n}{2^p}\rb^{2^p}       \,\cdot\,
            2^{p\cdot m \cdot n}
        \\ & \quad\quad\;\;\;
            \underbrace{\leq\,\,}_{p > \log m} 
            2^p                                     \,\cdot\,
            1                                        \,\cdot\,
            e^{m\cdot n}                             \,\cdot\,
            2^{p\cdot m \cdot n}
    \end{align*}
    And hence 
    \begin{equation}
        \log\, \gamma_{p, m, n}  
        \,\leq\, 
        p\cdot m\cdot n + p + m\cdot n\, \log e
        = Q_2\lb p, d\rb
    \end{equation}
    As we claimed \QED 
\end{proof}

\begin{remark}
    The intuition is that when $p$ become large enough, then increasing the depth can't increase 
    the amount of different summands anymore, since it is already maximal, and the bottleneck is in 
    the amount of different variables. Which is what forms the discussed trade-off.
\end{remark}

\subsection{Experiment details}
\subsubsection{Training details}
\paragraph{}
For each $B\in \ls 32K,\, 64K,\, 128K,\, 256K \rs$
and ratio $R \in \ls \frac{1}{4},\, \frac{1}{2},\, 1,\, 2,\, 4,\, 8\rs$,
 we defined $d\lb p, B\rb$ to be the rounded width appropriate for architecture 
 with depth $p$ and budget $B$, and taken $p$ to be  
 \equ{
    p \,=\, \underset{p}{\arg\min}\; 
    \ls\; p\;\; \Big{|}\;\; \frac{p}{\log_2\, d\lb p, B\rb} > R\;\rs 
 }
 We then trained the appropriate mixer model $y_{p,\, d}^{MM}$, 
 over CIFAR-100 for $40$ epochs, and calculated the final test accuracy 
 which we will denote by $\alpha_{B,\, R}$. 
 Finally we calculated the  best ratio by taking 
 $R_B^* = \underset{R}{\arg\max}\; \alpha_{B,\, R}$ 
 for each $B$. We repeat this experiment with six different seeds, and when 
 there is disagreement, we report the $R_B^*$ using majority, 
 the optimal resulted ratios are reported below 
 \begin{center}
\begin{tabular}{ |c|c|c|c|c| } 
 \hline
 Budget  & 32K & 64K &  128K & 256K \\
 \hline
 $R^{*}$   & .67 & 1.15 & 1.06 & 1.14\\
 \hline
\end{tabular}
\end{center}
This align with our theory predictions, about $1$ as optimal ratio, 
asymptotically in $B$. The ratios are not exact integers, 
due to the limitations we have in choosing $p, d$ to obey 
the given budget $B$, and the fact that both $p, d$ have to be integers, 
so it is practically impossible for the number $R=\frac{p}{\log_2\, d}$ 
to be every number, but we can make it pretty close.

\paragraph{}
Additionally we trained our model using, $128$ batch-size, and trained for $40$ 
epochs, we calculated the accuracy over the CIFAR-100 test set. 
We used $lr\,=\,10^{-3}$, and patch size of $4\times4$. 
We used the Adam optimizer, with $weight\_decay\,=\,5\cdot 10^{-5}$, 
and $\lb \beta_1,\, \beta_2\rb = \lb 0.9,\, 0.999\rb$. 
As augmentations we used random crop, and tensor normalization. 
And $dropout=0.5$ for the mlp layers.

\paragraph{}
Training each model for 40 epochs takes less then two hours, 
on our $RTX2060$ gpus. 
The experiment was launch using 144 parallel runs over RTX2060 gpus,  
over all the configurations of the form 
$\lb B,\, R,\, S\rb 
\in \mathbf{B}\times\mathbf{R}\times\mathbf{S}$ 
with $\abs{\mathbf{B}}=4$, $\abs{\mathbf{R}}=6$, and
$\abs{\mathbf{S}}=6$. 

\subsubsection{Error-bars}
\paragraph{}
The results deviation for different random seeds. 
Is relatively small and always bounded by $0.01$. 
When we define the deviation to be the max distance across 
$6$ different seeds from their average.

\begin{figure}[h]
\begin{subfigure}{0.48\textwidth}
    \includegraphics[width=0.95\linewidth]{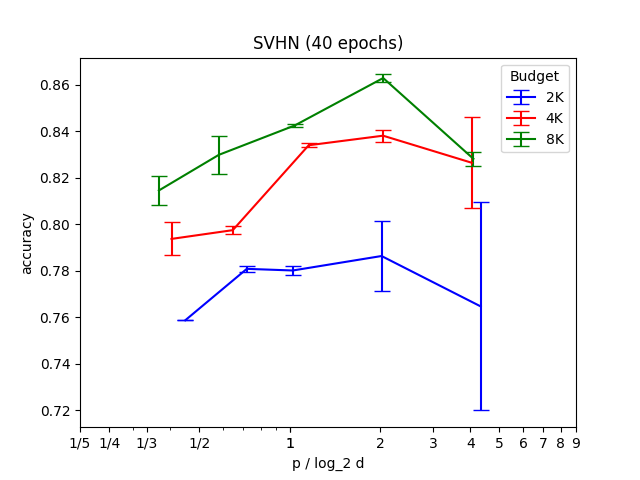} 
    \caption{SVHN}
    \label{fig:subim3}
\end{subfigure}
\begin{subfigure}{0.48\textwidth}
    \includegraphics[width=0.95\linewidth]{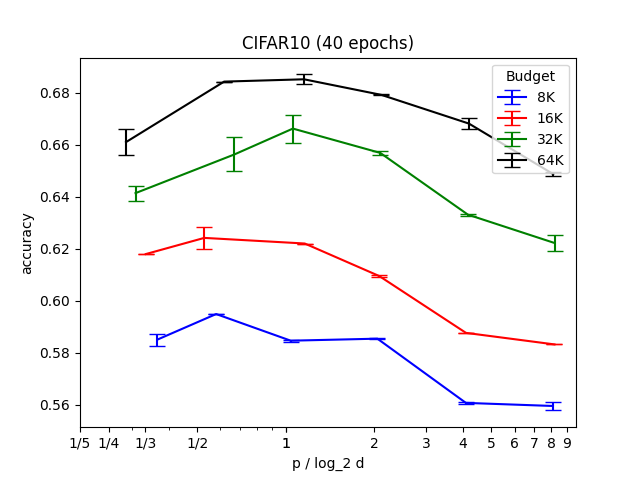} 
    \caption{CIFAR10}
    \label{fig:subim2}
\end{subfigure}
\begin{center}
\begin{subfigure}{0.48\textwidth}
    \includegraphics[width=0.95\linewidth]
    {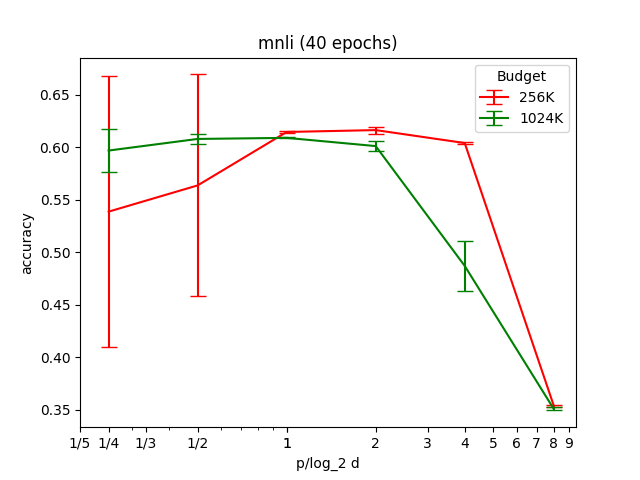} 
    \caption{MNLI}
    \label{fig:subim1}
\end{subfigure}    
\end{center}
\caption{Error bars for different parameter budget}
\label{fig:image3}
\end{figure}
