# Supplementary material for: Transformer Vs. MLP-Mixer: Exponential Expressive Gap For NLP Problems
Source: arXiv:2208.08191 source file (2022-11-17)
Supplement: Supplementary file 12 [file main.tex]

\documentclass{article}

% XXXXXXXXXXXXXXXXXXXXXXXXX
% TODO MY CHNAGE CHECK IF LEGITIMATE
\bibliographystyle{abbrvnat}
% XXXXXXXXXXXXXXXXXXXXXXXXX

% if you need to pass options to natbib, use, e.g.:
%     \PassOptionsToPackage{numbers, compress}{natbib}
% before loading neurips_2022
\usepackage[numbers]{natbib}


% ready for submission
\usepackage[preprint]{neurips_2022}


% to compile a preprint version, e.g., for submission to arXiv, add add the
% [preprint] option:
%     \usepackage[preprint]{neurips_2022}


% to compile a camera-ready version, add the [final] option, e.g.:
%     \usepackage[final]{neurips_2022}


% to avoid loading the natbib package, add option nonatbib:
%    \usepackage[nonatbib]{neurips_2022}


\usepackage[utf8]{inputenc} % allow utf-8 input
\usepackage[T1]{fontenc}    % use 8-bit T1 fonts
\usepackage{hyperref}       % hyperlinks
\usepackage{url}            % simple URL typesetting
\usepackage{booktabs}       % professional-quality tables
\usepackage{amsfonts}       % blackboard math symbols
\usepackage{nicefrac}       % compact symbols for 1/2, etc.
\usepackage{microtype}      % microtypography
\usepackage{xcolor}   % colors


\title{
Transformer Vs. MLP-Mixer: Exponential Expressive Gap For NLP Problems
}




%%%%%%%%%%%%%%%%%%%%% My packages %%%%%%%%%%%%%%%%%%%%%%%%%%%%

\usepackage{wrapfig}
\usepackage[export]{adjustbox}

%%%%%%%%%%%%%%%% My macro from ICLR %%%%%%%%%%%%%%%%%%%%%%%%%%


\newcommand{\epsbf}{{\boldsymbol{\varepsilon}}}
\newcommand{\eg}{\emph{e.g.}}
\newcommand{\ie}{\emph{i.e.}}
\newcommand{\cf}{\emph{cf.}}
\newcommand{\etc}{\emph{etc.}}
\newcommand{\wrt}{w.r.t.}
\newcommand{\dof}{d.o.f.}
\newcommand{\etal}{\emph{et al.}}
\newcommand*{\SQUEEZE}{}
\newcommand{\h}{{\mathbf h}}
\newcommand{\w}{{\mathbf w}}
\newcommand{\x}{{\mathbf x}}
\newcommand{\y}{{\mathbf y}}
\newcommand{\g}{{\mathbf g}}
\newcommand{\f}{{\mathbf f}}
\newcommand{\z}{{\mathbf z}}
\newcommand{\uu}{{\mathbf u}}
\newcommand{\s}{{\mathbf s}}
\newcommand{\e}{{\mathbf e}}
\newcommand{\aaa}{{\mathbf a}}
\newcommand{\bb}{{\mathbf b}}
\newcommand{\cc}{{\mathbf c}}
\newcommand{\dd}{{\mathbf d}}
\newcommand{\oo}{{\mathbf o}}
\newcommand{\p}{{\mathbf p}}
\newcommand{\K}{{\mathbf K}}
\newcommand{\Z}{{\mathbf Z}}
\newcommand{\0}{{\mathbf 0}}
\newcommand{\A}{{\mathcal A}}
\newcommand{\B}{{\mathcal B}}
\newcommand{\CC}{{\mathcal C}}
\newcommand{\D}{{\mathcal D}}
\newcommand{\F}{{\mathcal F}}
\newcommand{\G}{{\mathcal G}}
\newcommand{\HH}{{\mathcal H}}
\newcommand{\KK}{{\mathcal K}}
\newcommand{\M}{{\mathcal M}}
\newcommand{\NN}{{\mathcal N}}
\newcommand{\PP}{{\mathcal P}}
\newcommand{\T}{{\mathcal T}}
\newcommand{\X}{{\mathcal X}}
\newcommand{\Y}{{\mathcal Y}}
\newcommand{\OO}{{\mathcal O}}
\newcommand{\I}{{\mathcal I}}
\newcommand{\C}{{\mathbb C}}
\newcommand{\EE}{{\mathbb E}}
\newcommand{\V}{{\mathbb V}}
\newcommand{\N}{{\mathbb N}}
\newcommand{\SSS}{{\mathbb S}}
%%%%%%%%%%%%%%%%%%%%%%%%
\newcommand{\nocontentsline}[3]{}
\newcommand{\tocless}[2]{\bgroup\let\addcontentsline=\nocontentsline#1{#2}\egroup}
\newcommand{\alphabf}{{\boldsymbol{\alpha}}}
\newcommand{\betabf}{{\boldsymbol{\beta}}}
\newcommand{\gammabf}{{\boldsymbol{\gamma}}}
\newcommand{\lambdabf}{{\boldsymbol{\lambda}}}
\newcommand{\mubf}{{\boldsymbol{\mu}}}
\newcommand{\sigmabf}{{\boldsymbol{\sigma}}}
\newcommand{\psibf}{{\boldsymbol{\psi}}}
\newcommand{\abs}[1]{\left\lvert#1 \right\rvert}
\newcommand{\norm}[1]{\left\|#1 \right\|}
\newcommand{\indc}[1]{\mathbbm{1}\left[#1\right]}
\newcommand{\todo}[1]{\textcolor{red}{#1}}
\newcommand{\setprod}[2]{\underset{#1}{{\overset{#2}{\times}}}}
\newcommand{\shortminus}{\scalebox{0.8}[1]{-}}
\newcommand{\shortcdots}{\scalebox{0.5}[1]{\text{$\cdots$}}}
\newcommand{\mexu}[2]  {\underset{#2}{MEX_{#1}}}
\newcommand{\cupdot}{\mathbin{\mathaccent\cdot\cup}}
\newcommand{\otimesuo}[2]  {\underset{#1}{\overset{#2}{\otimes}}}
\newcommand{\odotuo}[2]  {\underset{#1}{\overset{#2}{\odot}}}
\newcommand\shorteq{\rule[.4ex]{3pt}{0.4pt}\llap{\rule[.8ex]{3pt}{0.4pt}}}
\newcommand{\mat}[1]{\llbracket#1\rrbracket}
\newcommand{\sep}[2]{\mathrm{sep}_{(#1)}\left( #2 \right)}
\newcommand{\rank}[1]{\mathrm{rank}\left( #1 \right)}
\newcommand{\trace}[1]{\mathrm{trace}\left( #1 \right)}
\newcommand{\matflex}[1]{\left\llbracket#1\right\rrbracket}
\renewcommand{\bibsection}{}
\newcommand{\simnets}{cohen2014simnets}
\newcommand{\deepsimnets}{cohen2015deep}
\newcommand{\cactd}{cohen2015expressive}
\newcommand{\crngtd}{cohen2016convolutional}
\newcommand{\tmm}{sharir2016tensorial}
\newcommand{\R}{\mathbb{R}}
\def\multiset#1#2{\ensuremath{\left(\kern-.3em\left(\genfrac{}{}{0pt}{}{#1}{#2}\right)\kern-.3em\right)}}
\newcommand{\q}{{\mathbf q}}
%%%%%%%%%%%%%%%%%%%%%%%%%%%%%%%%%%%
\def\be{\begin{equation}}
\def\ee{\end{equation}}
\def\beas{\begin{eqnarray*}}
\def\eeas{\end{eqnarray*}}
\def\bea{\begin{eqnarray}}
\def\eea{\end{eqnarray}}
%%%%%%%%%%%%%%%%% END ICLR MACROS %%%%%%%%%%%%%%%%%%%%%%%%%%%%%%%%%%%


%%%%%%%%%%%%%%TODAY%%%%%%%%%%%%%%%%%%%%
% MY MACROS
\usepackage{mathtools}

\newcommand{\mc}{\mathcal}
\newcommand{\defeq}{\vcentcolon=}
\newcommand{\eqdef}{=\vcentcolon}
\newcommand{\bigO}{\mathcal{O}}

\newtheorem{proofSketch}{Proof idea}[section]
\newtheorem{remark}{Remark}[section]
\newtheorem{theorem}{Theorem}[section]
\newtheorem{task}{Important-Task}[section]
\newtheorem{comment}{Comment}[section]
\newtheorem{importantComment}{Important Comment}[section]
\newtheorem{corollary}{Corollary}[theorem]
\newtheorem{summarizing}{Summarizing-Results}[theorem]
\newtheorem{result}{Result}[theorem]
\newtheorem{lemma}[theorem]{Lemma}
\newtheorem{claim}[theorem]{Claim}
\newtheorem{observation}[theorem]{Observation}
\newtheorem{conclusion}[theorem]{Conclusion}
\newtheorem{notation}[theorem]{Notation}
\newtheorem{definition}[theorem]{Definition}
\newtheorem{property}[theorem]{Property}
\newtheorem{proof}[theorem]{Proof}
\newtheorem{trial}[theorem]{Trial}
\newtheorem{proposition}[theorem]{Proposition}
\newtheorem{hypo}[theorem]{Hypothesis}
\newtheorem{LB}[theorem]{Lower Bound}
\newtheorem{concluding}[theorem]{To Conclude}
\newtheorem{assumption}[theorem]{Assumption}
\newtheorem{shortDescription}[theorem]{Short Description}
\newtheorem{note}[theorem]{Note}
%%%%%%%%%%%%%%%%%%%%%%%%%%%%%%%%%%%%%
\newcommand{\thm}[1]{\newtheorem{#1}[theorem]{#1}}
%%%%%%%%%%%%%%%%%%%%%%%%%%%%%%%%%%%%%


\def\lf{\left\lfloor}   
\def\rf{\right\rfloor}

\def\rb{\right)}
\def\lb{\left(}

\def\rc{\right]}
\def\lc{\left[}

\def\rs{\right\}}
\def\ls{\left\{}

\def\sep{\quad \bigwedge\quad}
\def\imp{\quad \implies\quad}
\def\txt#1{\quad\text{#1}\quad}

\def\f#1#2{#1\lb #2\rb}
\def\sum#1#2#3{\overset{#1}{\underset{#2}{\Sigma}} #3}
\def\pro#1#2#3{\overset{#1}{\underset{#2}{\prod}} #3}
\def\darrow{\begin{equation}
                \Downarrow
            \end{equation}}

\def\env#1#2{
    \begin{#1}
        #2
    \end{#1}
}

\def\abs#1{\left| #1\right|}


\def\Sol{F_\epsilon}
%%%%%%%%%%%%%%%%%%%%%%%%%%%%%%%%%%%%%
\usepackage{mathtools} 
\usepackage{changepage} 
%%%%%%%%%%%%%%%%%%%%%%%%%%%%%%%%%%%%%%


\def\ex{\mathbb{E}}
\def\D{\mathcal{D}}

%%%%%%%%%%%%%%%%%%%%%%%%%%%%%%%%%%%%%%
\usepackage{amssymb}
\newcommand{\QED}{
\textit{$\quad\quad\quad\quad\quad\quad\blacksquare$}
}

%%%%%%%%%%%%%%%%%%%%%%%%%%%%%%%%%%%%%%

\newcommand{\equ}[1]{
    \begin{equation}
        #1
    \end{equation}
}


%%%%%%%%%%%%%%%%%%%%%%%%%%%%%%%%%%%%%%

\usepackage{caption}
\usepackage{subcaption}

%%%%%%%%%%%%%%%%%%%%%%%%%%%%%%%%%%%%%%




%%%%%%%%%%%%%%%%%%%%%%%%%%%%%%%%%%%%%%%%%%%%%%%%%%%%%%%%%%%%%%%%%%%%%%


% The \author macro works with any number of authors. There are two commands
% used to separate the names and addresses of multiple authors: \And and \AND.
%
% Using \And between authors leaves it to LaTeX to determine where to break the
% lines. Using \AND forces a line break at that point. So, if LaTeX puts 3 of 4
% authors names on the first line, and the last on the second line, try using
% \AND instead of \And before the third author name.
\usepackage{authblk}




\author[]{
\textbf{Dan Navon}$^{1}$ $\quad\quad$
\textbf{Alex M. Bronstein}$^{2}$}

%$^1$ $\quad\quad$ 
%\textbf{Alex M. Bronstein}$^{2,\, 3}$}


\affil[1]{Department of Computer Science, The Hebrew University Of Jerusalem}
\affil[2]{Department of Computer Science, Technion
    Israel Institute Of Technology}
    
% \affil[3]{Sibylla, UK}
\affil[1]{\texttt{Dan.Nav@mail.huji.ac.il}}

\date{%
    $^1$Department of Computer Science, 
          The Hebrew University Of Jerusalem\\%
    $^2$Department of Computer Science, Technion\\[2ex]%
    \today
}

% \author {
%     Dan Navon,\textsuperscript{\rm 1, 2}
%     Alex M. Bronstein\textsuperscript{\rm 1}
% }
% \affiliations {
%     \textsuperscript{\rm 1} 
%     Department of Computer Science, Technion, Haifa, Israel\\
%     \textsuperscript{\rm 2} 
%     Department of Computer Science, The Hebrew University Of Jerusalem\\
%     dannav@technion.ac.il
% }



\begin{document}

\input{cvpr2023-author_kit-v1_1-1/appendix/body.tex}


%%%%%%%%%%%%%%%%%%%%%%%%%%%%%%%%%%%%%%%%%%%%%%%%%%%%%%%%%%%%
\newpage
\appendix
\tableofcontents

\input{appendix_A.tex}
\input{appendix_B.tex}
\input{appendix_C.tex}
\input{appendix_D.tex}
\input{appendix_E.tex}
\input{appendix_F.tex}
\input{appendix_G.tex}
\input{appendix_H.tex}
\input{appendix_I.tex}


%%%%%%%%%%%%%%%%%%%%%%%%%%%%%%%%%%%%%%%%%%%%%%%%%%%%%%%%%%%%

\end{document}
